# Supplementary material for: Evaluating Agentic Bioinformatics through Function, Evidence, and Validation
Source: arXiv:2607.27556 source file (2026-07-30)
Supplement: Supplementary file 1 [file Supplementary.tex]

\maketitle \section{Supplementary Section S1. Scope and Literature Selection Methodology} \label{sec:supplementary_methods} 

\textbf{Review design and scope.} This study presents a structured narrative review and evidence map of emerging agentic bioinformatics systems. The review was designed to support conceptual synthesis and cross-system comparison rather than exhaustive systematic coverage or meta-analysis. We use \emph{agentic bioinformatics} in a workflow-centered sense to describe computational systems that coordinate biological objectives, data, models, databases, software tools, and analytical actions across one or more stages of a scientific workflow. Systems were considered agentic or agent-adjacent when they demonstrated one or more substantive workflow-level capabilities beyond unconstrained conversational response generation. These capabilities included biological-goal interpretation, multi-step planning, task decomposition, adaptive retrieval, tool or code execution, workflow-state maintenance, error repair, evidence-grounded interpretation, verification, provenance capture, or coordination among specialized agents or modules. 

\textbf{Information sources and temporal scope.} Relevant studies were identified through targeted searches of PubMed, Google Scholar, Semantic Scholar, arXiv, bioRxiv, medRxiv, and major publisher or digital-library platforms, including Oxford Academic, Nature Portfolio, ACM, IEEE, and Elsevier. The primary search window covered January 2022 through July 2026. Earlier publications were retained when needed to contextualize bioinformatics workflow execution, reproducibility, provenance, retrieval, and verification. Peer-reviewed articles, conference papers, and preprints were included because many systems in this rapidly evolving field were initially reported outside archival journals. 

\textbf{Search strategy.} Searches combined terms describing agentic-computing paradigms with biological workflow domains. Agent-oriented terms included ``agentic bioinformatics'', ``biological LLM agents'', ``biomedical LLM agents'', ``multi-agent systems bioinformatics'', ``autonomous bioinformatics agent'', ``tool-augmented LLM bioinformatics'', and ``scientific discovery agents biology''. Domain-oriented terms covered genomics, transcriptomics, single-cell and spatial omics, proteomics, structural biology, protein design, gene editing, drug discovery, computational pathology, biological imaging, and general bioinformatics workflow automation. Additional searches used terms related to workflow execution, benchmarking, provenance, reproducibility, verification, error repair, and experimental validation. Backward and forward citation tracing, together with targeted system-name searches, was used to identify primary system papers, companion benchmarks, updated versions, and additional studies referenced by recent reviews. 

\textbf{Eligibility criteria.} We included AI-based systems, frameworks, benchmarks, or workflow infrastructures applied to biological or biomedical computational tasks when the publication reported sufficient information to characterize at least one workflow-relevant agentic function, evidence source, or validation procedure. The scope covered genomics, transcriptomics, multi-omics, single-cell and spatial biology, proteomics, structural biology, protein design, perturbation analysis, gene editing, drug discovery, therapeutic reasoning, computational pathology, biological imaging, biomedical data analysis, and general bioinformatics workflow automation. We excluded purely conversational or educational LLM applications without substantive retrieval, tool use, execution, verification, or evidence-grounded analysis; generic agents without a biological or biomedical application; and conventional fixed workflow engines that lacked adaptive biological-goal interpretation, planning, or workflow-level decision-making. Duplicate preprint and journal versions were consolidated under the most complete publication record. Systems spanning multiple application areas were assigned to the domain representing their primary workflow contribution to avoid duplicate system counts. 

\textbf{Counting and interpretation.} The final evidence map contains 109 agentic or agent-adjacent system entries and 28 benchmark or evaluation entries. Nine publications introduce both a system and an associated benchmark or evaluation resource; therefore, the complete map represents 128 unique publications. The system and benchmark counts describe the composition of this structured review sample and should not be interpreted as prevalence estimates in the complete literature.

\section{Supplementary Section S2. Domain-Specific FEV System Maps}

This section expands the representative mapping in the main text through domain-specific system tables. All tables use a common set of columns to compare demonstrated workflow Function, supporting Evidence, and reported use-case-specific Validation. The tables also retain the task scope, reported artifacts, provenance information, evaluation procedures, and principal limitations needed to interpret each classification. The extended mapping is organized into seven groups: Genomics, Transcriptomics, Perturbation, and CRISPR Agents; Single-Cell, Spatial Biology, Cell Annotation, and Spatial-Omics Agents; Proteomics, Structural Biology and Protein-Design Agents; Drug Discovery, Therapeutic Reasoning, and Molecular Design Agents; Computational Pathology, Microscopy, and Spatial Imaging Agents; General Bioinformatics Workflow Agents and Automation Systems; and Benchmarks, Evaluation Suites, and Workflow Infrastructure. Within each biological domain, systems are ordered according to their primary contribution to the workflow rather than alphabetically, chronologically, or by assumed maturity ranking. The tables generally progress from data access, metadata curation, retrieval, and interactive assistance to tool-mediated execution, analytical interpretation, diagnostic or discovery-oriented reasoning, and, where reported, prospective empirical evaluation. This ordering is intended to clarify differences in workflow scope; it does not imply that a later system is globally more capable, more reliable, or better validated than an earlier system. Systems spanning multiple domains are assigned to the section that best represents their principal contribution to workflow. Cross-domain capabilities are retained in their Function and Evidence profiles rather than represented through duplicate system entries whenever possible. Benchmark and evaluation resources are organized separately by evaluation scope, including evidence retrieval and verification, executable workflow completion, domain-specific analysis, robustness and failure assessment, artifact generation, and execution-trajectory evaluation. 
\paragraph{FEV profile notation.} Function profiles are coded as \textbf{F1}, planning and task decomposition; \textbf{F2}, role specialization and coordination; \textbf{F3}, tool selection and workflow execution; \textbf{F4}, workflow-state maintenance and trace capture; \textbf{F5}, self-evaluation and repair; and \textbf{F6}, verification and escalation. Evidence profiles are coded as \textbf{E1}, scientific literature; \textbf{E2}, structured biological knowledge; \textbf{E3}, biological measurements and metadata; \textbf{E4}, software and statistical outputs; \textbf{E5}, scientific-model outputs; and \textbf{E6}, experimental or clinical observations. Reported Validation stages are coded as \textbf{V0}, illustrative output; \textbf{V1}, demonstrated execution; \textbf{V2}, replayable computation; \textbf{V3}, scientifically evaluated computation; and \textbf{V4}, prospective empirical evaluation. Validation qualifiers are coded as \textbf{B}, quantitative benchmark or relevant baseline comparison; \textbf{H}, protocol-based human or expert assessment; \textbf{S}, statistical diagnostics, calibration, or uncertainty analysis; \textbf{R}, robustness, sensitivity, ablation, or failure analysis; \textbf{X}, external or independent validation; \textbf{P}, prospective empirical testing; and \textbf{C}, closed-loop empirical refinement. Function and Evidence codes are descriptive and non-ordinal. Reported V-stages and qualifiers apply to specific evaluated use cases and do not constitute global platform rankings. The V-stages are cumulative, and the qualifiers do not override the unmet cumulative-stage requirements. Qualifier \textbf{C} is assigned only when a newly generated empirical result is returned to the system and changes a subsequent computational or experimental action.

\subsection{Genomics, Transcriptomics, Perturbation, and CRISPR Agents} 

Tables~\ref{tab:genomics_agents_access}-- \ref{tab:genomics_agents_perturbation} map systems spanning genomic data access, transcriptomic analysis, evidence-grounded interpretation, diagnostic reasoning, perturbation design, and CRISPR experiment support. Representative tasks include sequencing-data processing, metadata extraction, genomic database querying, differential-expression and gene--trait analysis, gene-set and regulatory-network interpretation, rare-disease diagnosis, perturbation prioritization, and guide-RNA design. The mapped systems range from agent-adjacent extraction or prediction components to stateful, tool-executing workflows and experimentally connected gene-editing systems. 

Despite this diversity, the systems share several recurring workflow requirements, summarized in Figure~\ref{fig:genomics_crosscutting_fev_blueprint}. A biological objective must be translated into an appropriate analytical plan; sequencing, variant, phenotype, cohort, and perturbation data must be linked to their metadata; and domain tools must be selected and executed with traceable inputs, parameters, and outputs. Subsequent analyses may involve differential expression, association or survival modeling, regulatory-network inference, causal analysis, diagnostic prioritization, or perturbation-response prediction. Resulting claims should remain linked to identifiable molecular data, literature, databases, ontologies, pathways, and computational artifacts. 

Workflow-state maintenance, trace capture, verification, repair, and escalation operate in these activities rather than as isolated final steps. Their importance increases for diagnostic and intervention-oriented output, where errors in sample grouping, genome building, batch handling, variant identity, statistical assumptions, or evidence attribution can propagate into consequential conclusions. Prospective empirical testing remains optional and relatively uncommon; archived perturbation or clinical data contribute to the Evidence profile but do not establish prospective Validation of a newly generated recommendation. 

Table~\ref{tab:genomics_crosscutting_patterns} translates these recurring patterns into domain-specific design requirements. It identifies the molecular inputs, metadata, analytical artifacts, evidence links, execution records, verification outputs, and empirical readouts that should remain inspectable. Together, the system maps, the synthesis figure and the design-requirement table separate workflow functionality, evidentiary traceability, and use-case-specific validation.

% ============================================================ % Table 1: Retrieval, metadata, and foundational analysis % ============================================================ 
\begin{table*}[!t] \centering \footnotesize \caption{\textbf{Genomics, transcriptomics, perturbation, and CRISPR systems: retrieval, metadata, and foundational analysis.}} \label{tab:genomics_agents_access} \setlength{\tabcolsep}{2pt} \renewcommand{\arraystretch}{1.22} \begin{tabular}{ p{0.10\linewidth} p{0.12\linewidth} p{0.24\linewidth} p{0.24\linewidth} p{0.24\linewidth} } \hline \rowcolor{tableHeader} \textbf{System} & \textbf{Task} & \textbf{Function profile} & \textbf{Evidence profile} & \textbf{Reported V-stage and qualifiers} \\ \hline \flowlabel{flowAccessLabel} {Retrieval, Metadata, and Foundational Analysis} \rowcolor{flowAccess} ChIP-GPT \cite{cinquin2024chip} & ChIP-seq and SRA metadata extraction & \textbf{Agent-adjacent; F1, F5.} Structures extraction requests and iteratively resolves incomplete or inconsistent SRA metadata. & \textbf{E1, E2, E4.} SRA/GEO records, abstracts, protocols, expert labels, extracted fields, and model outputs. & \textbf{V1 [B,H].} Evaluated against curated metadata labels; replayable end-to-end analysis is not established. \\ \rowcolor{flowAccess} GeneGPT \cite{jin2024genegpt} & Genomic database QA and sequence alignment & \textbf{F1, F3.} Decomposes genomic questions into NCBI E-utilities or BLAST calls and combines returned records. & \textbf{E2, E4.} NCBI Gene, SNP, OMIM, Nucleotide, API calls, BLAST results, and returned identifiers. & \textbf{V2 [B].} Code, benchmark data, API trajectories, and returned records support replay of GeneTuring and GeneHop tasks. \\ \rowcolor{flowAccess} Nano Bio-Agent \cite{hong2025nano} & Small-model genomic question answering & \textbf{F1, F3, F4.} Classifies tasks, retrieves plans, infers parameters, executes APIs, and aggregates results through reusable templates. & \textbf{E2, E4, E5.} NCBI records, API outputs, execution traces, and small-language-model or AlphaGenome predictions. & \textbf{V1 [B,R].} Benchmarked across tasks, models, scales, runtime, memory, and cost; complete replayability is not established. \\ \rowcolor{flowAccess} ChatNT \cite{de2025multimodal} & Conversational biological-sequence prediction & \textbf{Agent-adjacent predictive component.} Performs language-conditioned DNA, RNA, and protein prediction without stateful tool orchestration. & \textbf{E3, E5.} Biological sequences, model predictions, confidence estimates, and feature attributions. & \textbf{V1 [B,S].} Evaluated on multitask prediction, calibration, and attribution benchmarks; V2 workflow replayability is not established. \\ \rowcolor{flowAccess} SeqMate \cite{mondal2024seqmate} & RNA-seq preprocessing and differential expression & \textbf{F1, F3.} Plans and executes preprocessing, alignment, quantification, differential expression, filtering, and reporting. & \textbf{E1, E2, E3, E4.} FASTQ files, sample metadata, reference genomes, QC reports, alignments, count matrices, differential-expression results, and retrieved knowledge. & \textbf{V1.} End-to-end execution is demonstrated, but versioned environments, complete parameters, traces, and replay checks are not reported. \\ \hline \end{tabular} \end{table*} % ============================================================ % Table 2: Executable transcriptomic workflows % ============================================================ 
\begin{table*}[!t] \centering \footnotesize \caption{\textbf{Genomics, transcriptomics, perturbation, and CRISPR systems: executable transcriptomic workflows.}} \label{tab:genomics_agents_execution} \setlength{\tabcolsep}{2pt} \renewcommand{\arraystretch}{1.22} \begin{tabular}{ p{0.10\linewidth} p{0.12\linewidth} p{0.24\linewidth} p{0.24\linewidth} p{0.24\linewidth} } \hline \rowcolor{tableHeader} \textbf{System} & \textbf{Task} & \textbf{Function profile} & \textbf{Evidence profile} & \textbf{Reported V-stage and qualifiers} \\ \hline \flowlabel{flowExecutionLabel} {Executable Transcriptomic Workflows} \rowcolor{flowExecution} GenoAgent \cite{liu2025genotex} & Gene-expression and gene--trait analysis & \textbf{F1, F2, F3, F4, F5.} Coordinates dataset selection, preprocessing, modelling, code review, debugging, and gene prioritization. & \textbf{E2, E3, E4.} GEO/TCGA data, clinical metadata, genomic databases, generated code, regression outputs, and ranked genes. & \textbf{V2 [B,R].} GenoTEX provides identifiable data, expert workflows, execution artifacts, quantitative evaluation, and ablations. \\ \rowcolor{flowExecution} GenoMAS \cite{liu2025genomas} & Code-driven gene--trait discovery & \textbf{F1, F2, F3, F4, F5.} Generates and executes analysis code while using shared state, review, backtracking, and correction. & \textbf{E2, E3, E4.} Expression and clinical data, identifier resources, generated code, statistical models, ranked genes, and review traces. & \textbf{V3 [B,S,R].} Evaluated through GenoTEX, confounder-aware modelling, execution analysis, baselines, ablations, and memory-reuse experiments. \\ \rowcolor{flowExecution} BIOGEN \cite{hossain2026biogen} & Evidence-grounded transcriptomic interpretation & \textbf{F1, F2, F4, F5, F6.} Coordinates retrieval, interpretation, and critics; preserves intermediate evidence and flags weak support. & \textbf{E1, E2, E3, E4.} RNA-seq modules, PubMed and UniProt records, enrichment outputs, semantic metrics, critic scores, and traceability reports. & \textbf{V3 [B,S,R,X].} A reproducible local implementation is evaluated on five bacterial RNA-seq datasets using baselines, grounding metrics, ablations, sensitivity analyses, and cross-organism tests. \\ \rowcolor{flowExecution} LLM4GRN \cite{afonja2025llm4grn} & Gene-regulatory-network inference & \textbf{Agent-adjacent; F1.} Generates candidate regulatory edges and combines them with statistical network inference. & \textbf{E2, E3, E4, E5.} Expression data, transcription-factor lists, biological knowledge, inferred networks, and synthetic-data outputs. & \textbf{V1 [B,S].} Evaluated using synthetic-data similarity and biological metrics; a replayable multistep workflow is not demonstrated. \\ \rowcolor{flowExecution} GeneAgent \cite{wang2025geneagent} & Gene-set interpretation with verification & \textbf{F1, F3, F5.} Generates interpretations, verifies claims through domain databases, and revises unsupported statements. & \textbf{E1, E2, E4.} Gene sets, pathway and disease databases, literature, enrichment outputs, and verification reports. & \textbf{V2 [B,H].} Evaluated on 1,106 gene sets with identifiable queries, verification outputs, quantitative metrics, and expert review. \\ \rowcolor{flowExecution} MRAgent \cite{xu2025mragent} & Mendelian-randomization causal analysis & \textbf{F1, F3, F4, F5, F6.} Retrieves GWAS data, executes MR analyses, checks reporting quality, and produces reviewed causal reports. & \textbf{E1, E2, E3, E4.} PubMed/PMC, OpenGWAS, UMLS, MR estimates, sensitivity analyses, STROBE-MR checks, and reports. & \textbf{V3 [B,H,S].} Evaluated across retrieval, dataset selection, statistical execution, sensitivity analysis, reporting, baselines, and expert review. \\ \rowcolor{flowExecution} AI-HOPE \cite{yang2025ai} & Clinical-genomic association and survival analysis & \textbf{F1, F3, F4.} Executes cohort selection, association testing, variable scanning, survival analysis, and reporting. & \textbf{E1, E3, E4.} TCGA genomic and clinical data, association statistics, odds ratios, hazard ratios, Kaplan--Meier outputs, and literature. & \textbf{V2 [S].} Provides executable analyses on identifiable retrospective datasets, but evaluation is limited to selected case studies. \\ \hline \end{tabular} \end{table*} % ============================================================ % Table 3: Diagnostic reasoning % ============================================================ 
\begin{table*}[!t] \centering \footnotesize \caption{\textbf{Genomics, transcriptomics, perturbation, and CRISPR systems: evidence-grounded diagnostic reasoning.}} \label{tab:genomics_agents_diagnosis} \setlength{\tabcolsep}{2pt} \renewcommand{\arraystretch}{1.22} \begin{tabular}{ p{0.10\linewidth} p{0.12\linewidth} p{0.24\linewidth} p{0.24\linewidth} p{0.24\linewidth} } \hline \rowcolor{tableHeader} \textbf{System} & \textbf{Task} & \textbf{Function profile} & \textbf{Evidence profile} & \textbf{Reported V-stage and qualifiers} \\ \hline \flowlabel{flowEvidenceLabel} {Evidence-Grounded Diagnostic Reasoning} \rowcolor{flowEvidence} HEAL-KGGen \cite{zuo2025heal} & Genetic-biomarker diagnostic QA & \textbf{F1, F2, F3, F5.} Routes questions to specialist agents, normalizes entities, retrieves knowledge-graph evidence, and verifies answers. & \textbf{E1, E2, E4.} Biomedical literature, medical knowledge graphs, retrieved subgraphs, and specialist-agent outputs. & \textbf{V2 [B].} Public code, requirements, test data, graph files, and instructions support replay of the evaluated QA setting. \\ \rowcolor{flowEvidence} RDguru \cite{yang2024rdguru} & Phenotype-grounded rare-disease diagnosis & \textbf{F1, F3, F4.} Normalizes phenotypes, combines diagnostic modules, maintains differential state, and selects follow-up questions. & \textbf{E1, E2, E3, E4, E5.} Clinical descriptions, HPO terms, rare-disease databases, retrieval outputs, and diagnostic rankings. & \textbf{V1 [B].} Evaluated on simulated and 238 retrospective cases; complete replayability and prospective clinical validation are not established. \\ \rowcolor{flowEvidence} MD2GPS \cite{zhou2025llm} & Mendelian diagnosis and gene prioritization & \textbf{F1, F2, F3, F5.} Coordinates variant annotation, gene--phenotype reasoning, and multi-agent debate to rank candidate genes. & \textbf{E2, E3, E4, E5.} VCF and HPO inputs, ClinVar/HGMD evidence, annotations, similarity scores, and ranked genes. & \textbf{V1 [B,X].} Evaluated on 1,185 samples across four datasets and 72 additional difficult cases; complete replayability is not established. \\ \rowcolor{flowEvidence} DeepRare \cite{zhao2026agentic} & Phenotype- and genotype-based rare-disease diagnosis & \textbf{F1, F2, F3, F4, F5, F6.} Coordinates phenotype, genotype, retrieval, and normalization services; maintains patient evidence and iteratively reassesses diagnoses. & \textbf{E1, E2, E3, E4, E5, E6.} Clinical narratives, HPO and WES/VCF data, confirmed diagnoses, literature, rare-disease resources, Exomiser results, variant rankings, and diagnostic hypotheses. & \textbf{V3 [B,H,R,X].} Public code and documented workflows support replay. Evaluation includes multi-centre datasets, diagnostic and physician baselines, specialist review, ablations, backbone comparisons, and failure analysis. \\ \hline \end{tabular} \end{table*} % ============================================================ % Table 4: Perturbation and CRISPR systems % ============================================================ 
\begin{table*}[!t] \centering \footnotesize \caption{\textbf{Genomics, transcriptomics, perturbation, and CRISPR agents: perturbation prediction, experiment design, and gene-editing intervention.} Reported V-stages follow the cumulative V0--V4 criteria.} \label{tab:genomics_agents_perturbation} \setlength{\tabcolsep}{2pt} \renewcommand{\arraystretch}{1.22} \begin{tabular}{ p{0.10\linewidth} p{0.12\linewidth} p{0.24\linewidth} p{0.24\linewidth} p{0.24\linewidth} } \hline \rowcolor{tableHeader} \textbf{System} & \textbf{Task} & \textbf{Function profile} & \textbf{Evidence profile} & \textbf{Reported V-stage and qualifiers} \\ \hline \flowlabel{flowDiscoveryLabel} {Perturbation-Response Prediction} \rowcolor{flowDiscovery} CausalPert \cite{martell2026causalpert} & Gene-perturbation response prediction & \textbf{F1, F2, F5.} Generates and aggregates regulatory hypotheses and selects anchor genes for response prediction. & \textbf{E2, E3, E4, E5, E6.} Interaction networks, archived Perturb-seq profiles, predicted regulators, confidence scores, and consensus rankings. & \textbf{V1 [B,R].} Evaluated retrospectively across four cell lines using baselines, low-data experiments, and ablations; V2 replayability is not established. \\ \rowcolor{flowDiscovery} PBIO-AGENT \cite{kim2026progressive} & Chemical and genetic response prediction & \textbf{F1, F2, F4, F5.} Coordinates mechanism, network, synthesis, and judge agents while propagating high-confidence reasoning traces. & \textbf{E2, E3, E4, E5, E6.} Biological networks, LINCS and Perturb-seq data, predicted responses, confidence measures, and candidate rankings. & \textbf{V1 [B,R].} Evaluated on LINCSQA and PerturbQA with multiple baselines and component analyses; complete replayability is not established. \\ \flowlabel{flowDiscoveryLabel} {Perturbation Experiment Design} \rowcolor{flowDiscovery} BioDiscoveryAgent \cite{roohani2025biodiscoveryagent} & Single-gene and combinatorial perturbation design & \textbf{F1, F3, F4, F5.} Plans sequential screens, searches literature and pathways, analyzes previous results, and revises candidates through critique. & \textbf{E1, E2, E3, E4, E6.} PubMed, Reactome, archived perturbation screens, phenotypic scores, hit curves, candidate lists, and critic outputs. & \textbf{V3 [B,S,R,X].} Public artifacts support replay. Evaluation spans multiple screens, repeated runs, Bayesian, random, and human baselines, tool ablations, and single-gene and combinatorial tasks. Rounds use archived outcomes, so P and C are not assigned. \\ \rowcolor{flowDiscovery} PerTurboAgent \cite{hao2025perturboagent} & Sequential Perturb-seq panel design & \textbf{F1, F3, F4, F5.} Selects CRISPRi panels through prediction, enrichment, reflection, refinement, and action memory. & \textbf{E2, E3, E4, E5, E6.} Archived Perturb-seq data, pathway resources, embeddings, enrichment outputs, predictions, action logs, and hit curves. & \textbf{V1 [B,R].} Evaluated retrospectively on 11 phenotype tasks using active-learning baselines and ablations; rounds are simulated and V2 replayability is not established. \\ \flowlabel{flowClosureLabel} {Prospective Gene-Editing Intervention} \rowcolor{flowClosure} CRISPR-GPT \cite{qu2026crispr} & CRISPR experiment design and analysis & \textbf{F1, F2, F3, F4, F5, F6.} Plans editing workflows, coordinates specialists, selects modalities and delivery strategies, invokes design tools, and supports expert oversight. & \textbf{E1, E2, E4, E6.} CRISPR literature and protocols, Primer3, CRISPRitz, CRISPResso2, and prospective knockout and activation measurements. & \textbf{V4 [B,H,P].} GeneEditingBench and expert evaluation are combined with prospective knockout and activation experiments. C is not assigned because assay feedback did not drive a subsequent editing round. \\ \hline \end{tabular} \end{table*}

\begin{table*}[!t] \centering \footnotesize \caption{\textbf{Cross-cutting design requirements for genomics, transcriptomics, perturbation, and CRISPR agents.} The requirements distinguish workflow Function, inspectable Evidence, and use-case-specific Validation.} \label{tab:genomics_crosscutting_patterns} \setlength{\tabcolsep}{3pt} \renewcommand{\arraystretch}{1.18} \begin{tabular}{ p{0.18\linewidth} p{0.28\linewidth} p{0.28\linewidth} p{0.2\linewidth} } \hline \rowcolor{tableHeader} \textbf{Workflow requirement} & \textbf{Domain-specific principle} & \textbf{Inspectable evidence and artifacts} & \textbf{FEV interpretation} \\ \hline \rowcolor{flowAccess} Genomic objective and planning & Define the sequencing, association, diagnostic, perturbation, or gene-editing objective and its analytical steps. & Research question, assay requirements, workflow plan, constraints, endpoints, and decision points. & \textbf{F1.} Planning defines the workflow but does not establish execution or validity. \\ \rowcolor{flowAccess} Analytical role coordination & Coordinate molecular-data processing, statistical analysis, biological interpretation, review, and experimental oversight. & Agent assignments, shared state, analytical handoffs, critic outputs, review notes, and approval records. & \textbf{F2.} Coordination does not independently establish reliability or a higher V-stage. \\ \rowcolor{flowAccess} Molecular data grounding & Resolve samples, assays, genome builds, phenotypes, cohorts, batches, treatments, and perturbation conditions. & FASTQ/BAM files, count matrices, SRA/GEO accessions, VCF/WES records, HPO terms, cohort metadata, and perturbation measurements. & \textbf{E3.} Traceable molecular inputs are necessary, but not sufficient, for replayability. \\ \rowcolor{flowExecution} Genomics tool execution & Run preprocessing, alignment, quantification, variant annotation, enrichment, database queries, guide design, and editing analysis. & Commands, parameters, logs, intermediate files, and outputs from tools such as HISAT, featureCounts, ANNOVAR, Exomiser, Primer3, CRISPRitz, and CRISPResso2. & \textbf{F3; E4.} Execution supports V1; V2 additionally requires replayable inputs, environments, parameters, and traces. \\ \rowcolor{flowExecution} Statistical and mechanistic analysis & Evaluate expression, association, survival, regulation, causality, diagnostic ranking, and perturbation response. & Differential-expression results, regression and survival models, regulatory networks, variant rankings, model predictions, and perturbation scores. & \textbf{E4; E5} for predictive or generative models. Scientific adequacy requires separate evaluation. \\ \rowcolor{flowEvidence} Evidence-grounded interpretation & Link genes, variants, pathways, phenotypes, diagnoses, and perturbation effects to identifiable biological sources. & PubMed, OMIM, ClinVar, HPO, GO, KEGG, Reactome, UniProt, database identifiers, retrieved passages, and evidence-linked reports. & \textbf{E1; E2.} Source access supports attribution but does not itself establish Validation. \\ \rowcolor{flowEvidence} Genomic trace capture & Preserve molecular inputs, analytical decisions, software execution, failures, repairs, and output lineage. & Accessions, sample identities, genome builds, software versions, parameters, scripts, notebooks, intermediate artifacts, and repair logs. & \textbf{F4; E4.} Trace capture supports V2 only when the evaluated workflow can be reconstructed or replayed. \\ \rowcolor{flowEvidence} Verification and escalation & Check sample grouping, batch effects, QC, model assumptions, identifiers, evidence attribution, uncertainty, and claim sufficiency. & QC and batch reports, sensitivity analyses, critic outputs, repaired code, evidence checks, uncertainty flags, and expert-review records. & \textbf{F5; F6.} Verification effectiveness must be established through task-appropriate Validation. \\ \rowcolor{flowClosure} Prospective perturbation or editing validation & Test an agent-generated gene, perturbation, guide RNA, editing protocol, diagnostic claim, or intervention recommendation. & Guide sequences, assay protocols, knockout or activation measurements, editing-efficiency results, functional readouts, and experimental records. & \textbf{E6; P.} V4 also requires the lower cumulative gates; \textbf{C} requires empirical feedback to change a subsequent action. \\ \hline \end{tabular} \vspace{0.3em} \begin{minipage}{0.98\textwidth} \footnotesize \textit{Note.} Requirements 1--6 define the core workflow in Figure~\ref{fig:genomics_crosscutting_fev_blueprint}; requirements 7--8 operate across that workflow. Requirement 9 is optional. Archived experimental or clinical observations contribute to Evidence but not to prospective Validation unless an output of the evaluated workflow is directly tested. \end{minipage} \end{table*}

\begin{figure*}[!t] \centering \resizebox{0.92\textwidth}{!}{% 
\begin{tikzpicture}[ x=4.45cm, y=1.0cm, core/.style={ rectangle, rounded corners, draw=blue!65!black, thick, fill=blue!7, text width=3.55cm, minimum height=1.30cm, align=center, font=\scriptsize }, evidenceband/.style={ rectangle, rounded corners, draw=green!55!black, thick, fill=green!7, text width=12.35cm, minimum height=0.92cm, align=center, font=\scriptsize }, control/.style={ rectangle, rounded corners, draw=orange!70!black, thick, fill=orange!8, text width=12.35cm, minimum height=0.88cm, align=center, font=\scriptsize }, empirical/.style={ rectangle, rounded corners, draw=red!65!black, thick, dashed, fill=red!5, text width=8.40cm, minimum height=0.96cm, align=center, font=\scriptsize }, sectionlabel/.style={ anchor=east, text width=1.95cm, align=right, font=\bfseries\scriptsize }, arrow/.style={ -{Latex[length=2mm]}, thick } ] % ============================================================ % Requirements 1--3: workflow formulation and input grounding % ============================================================ 
% ============================================================ % Requirements 1--3: workflow formulation and input grounding % ============================================================ 
\node[core] (planning) at (0,0) { \textbf{1. Genomic objective and planning}\\[0.18em] Define the sequencing, association, diagnostic, perturbation, or gene-editing task }; \node[core] (coordination) at (1,0) { \textbf{2. Analytical role coordination}\\[0.18em] Coordinate data processing, statistical modelling, biological review, and oversight }; \node[core] (grounding) at (2,0) { \textbf{3. Molecular data grounding}\\[0.18em] Resolve samples, assays, genome builds, phenotypes, cohorts, batches, and perturbation conditions }; \draw[arrow] (planning) -- (coordination); \draw[arrow] (coordination) -- (grounding); \node[ sectionlabel, text=blue!65!black ] at ([xshift=-0.35cm]planning.west) {Workflow\\formulation}; % ============================================================ % Requirements 4--6: domain-specific workflow operation % ============================================================ 
\node[core] (interpretation) at (0,-2.20) { \textbf{6. Genomic interpretation}\\[0.18em] Ground genes, variants, pathways, diagnoses, and perturbation effects in traceable evidence }; \node[core] (analysis) at (1,-2.20) { \textbf{5. Statistical and causal analysis}\\[0.18em] Evaluate differential expression, gene--trait associations, survival, regulation, and perturbation response }; \node[core] (execution) at (2,-2.20) { \textbf{4. Genomics tool execution}\\[0.18em] Run alignment, quantification, variant annotation, enrichment, database queries, and guide design }; \draw[arrow] (grounding.south) -- (execution.north); \draw[arrow] (execution) -- (analysis); \draw[arrow] (analysis) -- (interpretation); \node[ sectionlabel, text=blue!65!black ] at ([xshift=-0.35cm]interpretation.west) {Workflow\\operation}; % ============================================================ % Shared domain evidence and artifacts % ============================================================ 
\node[evidenceband] (artifacts) at (1,-4.05) { \textbf{Shared genomic evidence and artifacts:} FASTQ/BAM files, count matrices, SRA/GEO records, VCF/WES files, HPO and cohort metadata, database records, QC outputs, differential-expression results, variant annotations, fitted models, ranked genes, guide designs, and evidence-linked reports }; \node[ sectionlabel, text=green!45!black ] at ([xshift=-0.35cm]artifacts.west) {Shared genomic evidence\\and artifacts}; % ============================================================ % Requirements 7--8: cross-cutting controls % ============================================================ 
\node[control] (trace) at (1,-5.50) { \textbf{7. Genomic trace capture:} record accessions, sample identities, genome builds, database and software versions, parameters, code, intermediate artifacts, failures, repairs, and output lineage }; \node[control] (verification) at (1,-6.72) { \textbf{8. Genomic verification and escalation:} check sample grouping, batch effects, QC, model assumptions, identifiers, evidence support, and uncertainty; revise or escalate unsupported claims }; \node[ sectionlabel, text=orange!70!black ] at ([xshift=-0.35cm]trace.west) {Cross-cutting across\\requirements 1--6}; % ============================================================ % Requirement 9: optional empirical extension % ============================================================
\node[empirical] (empirical) at (1,-8.35) { \textbf{9. Optional perturbation or editing validation}\\[0.15em] Test prioritized genes, perturbations, guide RNAs, diagnostic claims, or editing protocols. Closed-loop refinement requires the result to guide a subsequent action }; \node[ sectionlabel, text=red!65!black ] at ([xshift=-0.35cm]empirical.west) {Optional empirical\\extension};============================================================ % Background groupings % ============================================================ 
\begin{pgfonlayer}{background} \node[ rectangle, rounded corners, draw=blue!22, fill=blue!1, fit=(planning)(coordination)(grounding), inner sep=0.15cm ] {}; \node[ rectangle, rounded corners, draw=blue!22, fill=blue!1, fit=(interpretation)(analysis)(execution), inner sep=0.15cm ] {}; \node[ rectangle, rounded corners, draw=orange!25, fill=orange!1, fit=(trace)(verification), inner sep=0.16cm ] {}; \end{pgfonlayer} \end{tikzpicture}% 
} \vspace{-0.2em} \caption{\textbf{Cross-cutting workflow blueprint for genomics, transcriptomics, perturbation, and CRISPR agents.} The blueprint summarizes the domain-specific requirements in Table~\ref{tab:genomics_crosscutting_patterns}. The core trajectory progresses from formulation of a sequencing, association, diagnostic, perturbation, or gene-editing objective to molecular-data grounding, execution of genomics tools and databases, statistical or mechanistic analysis, and evidence-linked interpretation. Genomic evidence and artifacts are used or generated across this trajectory. State and trace capture preserve sample, genome, software, parameter, and artifact lineage, while verification checks data quality, analytical assumptions, identifier consistency, evidentiary support, and uncertainty. Prospective perturbation or editing validation is optional. It constitutes closed-loop refinement only when the resulting empirical evidence changes a subsequent workflow action.} \label{fig:genomics_crosscutting_fev_blueprint} \end{figure*}

\subsection{Single-Cell, Spatial Biology, Cell Annotation, and Spatial-Omics Agents} 

Tables~\ref{tab:single_cell_agents_access}--\ref{tab:single_cell_agents_knowledge} map systems spanning single-cell data access, spatial-omics analysis, cell-type annotation, trajectory inference, cell--cell interaction modelling, perturbation prediction, and autonomous biological discovery. Representative tasks include public scRNA-seq dataset reuse, metadata extraction, preprocessing and integration, reference-free annotation, spatial-region analysis, ligand--receptor inference, pseudotime reconstruction, perturbation-response modelling, and multiomic hypothesis generation. The mapped systems range from natural-language data interfaces to stateful agents that execute, evaluate, and repair single-cell and spatial workflows. Despite this diversity, the systems share several recurring workflow requirements, summarized in Figure~\ref{fig:singlecell_spatial_crosscutting_fev_blueprint}. 

Single-cell or spatial data must first be linked to their assay, sample, tissue, species, condition, cohort, and study metadata. Cells and tissue regions must then be represented through expression states, markers, clusters, spatial coordinates, neighborhoods, tissue domains, and perturbation contexts. Domain tools are subsequently executed for preprocessing, integration, annotation, trajectory inference, cell--cell communication, segmentation, registration, and spatial analysis. Resulting annotations and biological claims should remain linked to marker evidence, reference atlases, pathway resources, literature, analytical outputs, and spatial context. Workflow-state maintenance, uncertainty assessment, critique, repair, verification, and provenance-preserving reporting operate across these activities rather than as isolated final steps. Their importance increases when systems infer cell identities, developmental trajectories, regulatory programs, ligand--receptor interactions, perturbation responses, or disease-associated spatial regions. Errors in sample metadata, batch handling, marker selection, spatial alignment, neighborhood construction, or annotation confidence can propagate into unsupported biological conclusions. Prospective testing remains optional and relatively uncommon; archived perturbation, spatial, or clinical observations contribute to the Evidence profile but do not establish prospective Validation of a newly generated result. 

Table~\ref{tab:singlecell_spatial_crosscutting_patterns} translates these recurring patterns into domain-specific design requirements. It identifies the expression objects, sample metadata, marker tables, spatial coordinates, neighborhood graphs, analytical outputs, annotation scores, workflow traces, evidence links, and empirical readouts that should remain inspectable. Together, the system maps, synthesis figure, and design-requirement table separate workflow functionality, evidentiary traceability, and use-case-specific validation.

% ============================================================ % Table 6: Data access and executable workflows % ============================================================ 
\begin{table*}[!t] \centering \footnotesize \caption{\textbf{Single-cell and spatial-omics agents: data access and executable workflows.}} \label{tab:single_cell_agents_access} \setlength{\tabcolsep}{2pt} \renewcommand{\arraystretch}{1.22} \begin{tabular}{ p{0.10\linewidth} p{0.12\linewidth} p{0.24\linewidth} p{0.24\linewidth} p{0.24\linewidth} } \hline \rowcolor{tableHeader} \textbf{System} & \textbf{Task} & \textbf{Function profile} & \textbf{Evidence profile} & \textbf{Reported V-stage and qualifiers} \\ \hline \flowlabel{flowAccessLabel} {Data Access and Standardization} \rowcolor{flowAccess} SRAgent \cite{youngblut2025scbasecount} & Agent-curated scRNA-seq repository & \textbf{F1, F3, F4, F5.} Discovers 10X scRNA-seq studies, extracts metadata, and routes raw reads through standardized Nextflow/STARsolo workflows. & \textbf{E2, E3, E4.} SRA accessions and metadata, raw reads, chemistry assignments, processed count matrices, workflow logs, and CELLxGENE comparisons. & \textbf{V3 [B,S,R,X].} Public code and data support replay; large-scale evaluation spans more than 230 million cells, 21 organisms, and 72 tissues, with analyses of processing consistency and technical confounding. \\ \rowcolor{flowAccess} CellAtria \cite{nouri2026agentic} & Document-to-analysis scRNA-seq reuse & \textbf{F1, F3, F4.} Extracts study metadata, resolves GEO accessions, retrieves datasets, and launches standardized CellExpress workflows. & \textbf{E1, E2, E3, E4.} Research articles, GEO metadata, sample annotations, AnnData objects, workflow records, and HTML reports. & \textbf{V2 [R].} Executable retrieval and standardized analysis artifacts support replay; biological evaluation remains limited. \\ \rowcolor{flowAccess} CompBioAgent \cite{zhang2025compbioagent} & Natural-language scRNA-seq exploration & \textbf{F1, F3.} Converts biological questions into CellDepot queries and Cellxgene VIP visualization requests. & \textbf{E2, E3, E4.} Public scRNA-seq datasets, structured queries, UMAPs, violin plots, heatmaps, and filtered cell-level outputs. & \textbf{V1.} Interactive data access and visualization are demonstrated, but systematic replay and scientific evaluation are not established. \\ \flowlabel{flowExecutionLabel} {Executable Single-Cell and Spatial Workflows} \rowcolor{flowExecution} BioInformatics Agent (BIA) \cite{xin2024bioinformatics} & End-to-end scRNA-seq analysis & \textbf{F1, F3, F4, F5.} Retrieves datasets and metadata, generates and executes Scanpy workflows, repairs failures, and produces analytical reports. & \textbf{E1, E2, E3, E4.} ENA/GEO/ArrayExpress records, FASTQ and AnnData inputs, metadata, QC outputs, clusters, annotations, interaction results, and pseudotime. & \textbf{V2 [B,R].} Demonstrates executable workflows and high metadata-extraction accuracy across 11 tasks; broader scientific evaluation remains limited. \\ \rowcolor{flowExecution} CellAgent \cite{xiao2024cellagent} & Automated single-cell and spatial analysis & \textbf{F1, F2, F3, F4, F5.} Coordinates planning, execution, and evaluation agents to select tools, parameters, and revised workflows. & \textbf{E2, E3, E4.} Single-cell and spatial datasets, workflow traces, clustering, marker, annotation, and downstream-analysis outputs. & \textbf{V3 [B,H,R].} Evaluated across single-cell tasks against computational workflows and human experts, with iterative optimization analyses. \\ \rowcolor{flowExecution} STAT \cite{chen2026stat} & Integrated spatial transcriptomics analysis & \textbf{F1, F3, F4, F5, F6.} Maintains a persistent spatial session, selects compatible skills, executes code, reflects on errors, interprets regions, and exports notebooks. & \textbf{E1, E2, E3, E4.} Visium, MERFISH, Xenium, and Visium HD data; H\&E images, ROI annotations, tool outputs, spatial statistics, notebooks, and reports. & \textbf{V3 [B,S,R,X].} Evaluated across 11 task categories, multiple platforms and resolutions, with baselines, backbone ablations, and reproduction of a published study. \\ \hline \end{tabular} \end{table*} % ============================================================ % Table 7: Spatial execution and annotation % ============================================================ 
\begin{table*}[!t] \centering \footnotesize \caption{\textbf{Single-cell and spatial-omics agents: spatial execution, annotation, and uncertainty.}} \label{tab:single_cell_agents_annotation} \setlength{\tabcolsep}{2pt} \renewcommand{\arraystretch}{1.22} \begin{tabular}{ p{0.10\linewidth} p{0.12\linewidth} p{0.24\linewidth} p{0.24\linewidth} p{0.24\linewidth} } \hline \rowcolor{tableHeader} \textbf{System} & \textbf{Task} & \textbf{Function profile} & \textbf{Evidence profile} & \textbf{Reported V-stage and qualifiers} \\ \hline \flowlabel{flowExecutionLabel} {Executable Spatial-Omics Workflows} \rowcolor{flowExecution} SpatialAgent \cite{wang2025spatialagent} & Autonomous spatial-biology analysis & \textbf{F1, F3, F4, F5, F6.} Plans and executes workflows for gene-panel design, annotation, cell--cell communication, reporting, and hypothesis generation. & \textbf{E1, E2, E3, E4.} Visium, MERFISH and Xenium data, marker databases, pathway resources, annotations, communication outputs, and reports. & \textbf{V3 [B,H,R,X].} Evaluated across tissues and species against computational baselines and human experts; prospective wet-lab validation is not established. \\ \rowcolor{flowExecution} STAgent \cite{lin2025spatial} & Spatial analysis and visual reasoning & \textbf{F1, F3, F4, F5.} Combines planning, code retrieval, Python execution, visual reasoning, literature retrieval, and autonomous reporting. & \textbf{E1, E2, E3, E4.} STARmap expression and coordinate data, spatial maps, Scanpy/Squidpy outputs, interaction analyses, retrieved literature, and reports. & \textbf{V3 [B,R,X].} Reproduces major spatial analyses and published findings across developmental time points; conclusions remain computational. \\ \rowcolor{flowExecution} SP-Mind \cite{yuansp} & Spatial-proteomics workflow automation & \textbf{F1, F3, F4, F5.} Uses curated skills, tool execution, failure diagnosis, and self-correction for multiplexed tissue-imaging workflows. & \textbf{E2, E3, E4.} CODEX, CyCIF, MIBI, and IMC data; registration, segmentation, quantification, clustering, and annotation outputs. & \textbf{V3 [B,R,X].} Evaluated on 102 SP-Bench tasks with quantitative execution and annotation metrics; performance depends on curated skill templates. \\ \flowlabel{flowEvidenceLabel} {Annotation, Evidence, and Uncertainty} \rowcolor{flowEvidence} scExtract \cite{wu2025scextract} & Published-data annotation and integration & \textbf{F1, F3, F4.} Extracts study metadata, configures preprocessing, annotates cells, and integrates datasets using publication-derived priors. & \textbf{E1, E2, E3, E4.} Research articles, AnnData objects, extracted metadata, marker evidence, annotation outputs, integration results, and reference benchmarks. & \textbf{V3 [B,R,X].} Outperforms reference-transfer baselines and integrates 14 datasets into a 440,000-cell human skin atlas. \\ \rowcolor{flowEvidence} Lightweight ST LLM Agent \cite{dip2025can} & Spatial-region annotation & \textbf{F2, F5.} Combines prototype niche cards, low-confidence LLM correction, multi-role review, spatial checks, and graph smoothing. & \textbf{E2, E3, E4, E5.} STARmap and MERFISH data, marker profiles, spatial neighborhoods, annotation predictions, and clustering metrics. & \textbf{V1 [B,S,R].} Benchmarked on six datasets using NMI, ARI, CHAOS, and ASW; agentic variants mostly match deterministic baselines, and replayability is not established. \\ \rowcolor{flowEvidence} CASSIA \cite{xie2025cassia} & Reference-free cell-type annotation & \textbf{F1, F2, F5, F6.} Generates competing annotations, validates marker support, scores quality, merges labels, and reports uncertainty. & \textbf{E1, E2, E3, E4, E5.} Marker tables, reference knowledge, annotation hypotheses, quality scores, uncertainty estimates, subclusters, and HTML reports. & \textbf{V3 [B,S,R,X].} Broadly benchmarked across cell types and tissues with quality scoring and annotation refinement; biological validation remains computational. \\ \rowcolor{flowEvidence} TACTIC \cite{alsabbagh2025tactic} & Explainable spatial cell-type annotation & \textbf{F1, F2, F5.} Combines expression, marker and spatial embeddings with junior--senior agent review to assign labels and confidence. & \textbf{E2, E3, E4, E5.} MERFISH, MIBI-TOF and Stereo-seq data, marker genes, spatial graphs, embeddings, annotations, and classification metrics. & \textbf{V3 [B,S,R,X].} Evaluated across three spatial platforms with quantitative annotation metrics and structural ablations; revised labels lack prospective testing. \\ \hline \end{tabular} \end{table*} % ============================================================ % Table 8: Trajectory and perturbation modeling % ============================================================ 
\begin{table*}[!t] \centering \footnotesize \caption{\textbf{Single-cell and spatial-omics agents: trajectory, interaction, and perturbation modelling.}} \label{tab:single_cell_agents_modeling} \setlength{\tabcolsep}{2pt} \renewcommand{\arraystretch}{1.22} \begin{tabular}{ p{0.10\linewidth} p{0.12\linewidth} p{0.24\linewidth} p{0.24\linewidth} p{0.24\linewidth} } \hline \rowcolor{tableHeader} \textbf{System} & \textbf{Task} & \textbf{Function profile} & \textbf{Evidence profile} & \textbf{Reported V-stage and qualifiers} \\ \hline \flowlabel{flowEvidenceLabel} {Annotation and Uncertainty} \rowcolor{flowEvidence} CyteType \cite{ahuja2025multi} & Uncertainty-aware cell-type annotation & \textbf{F1, F2, F5, F6.} Builds cluster context, generates competing cell-type hypotheses, validates marker evidence, detects heterogeneity, and reports confidence. & \textbf{E1, E2, E3, E4, E5.} Expression profiles, marker and ontology resources, pathway evidence, annotation hypotheses, confidence scores, and semantic-similarity metrics. & \textbf{V3 [B,S,R,X].} Evaluated across 205 clusters and 16 model backbones against established annotation methods, with confidence and heterogeneity analyses. \\ \flowlabel{flowEvidenceLabel} {Trajectory, Interaction, and Regulatory Modelling} \rowcolor{flowEvidence} SpaCellAgent \cite{wang2026spacellagent} & Single-cell and spatial trajectory inference & \textbf{F1, F3, F4, F5.} Generates, executes, evaluates, and repairs trajectory workflows while retaining validated templates. & \textbf{E1, E3, E4.} Single-cell and spatial datasets, executable code, pseudotime orderings, lineage topologies, evaluator feedback, plots, and reports. & \textbf{V3 [B,S,R,X].} Benchmarked across real and synthetic datasets against trajectory-inference baselines using topology, ordering, and efficiency metrics. \\  \flowlabel{flowDiscoveryLabel} {Perturbation and Multiomic Modelling} \rowcolor{flowDiscovery} HarmonyCell \cite{huang2026harmonycell} & Virtual-cell perturbation modelling & \textbf{F1, F3, F4, F5.} Harmonizes perturbation metadata and searches model architectures through adaptive MCTS and execution feedback. & \textbf{E2, E3, E4, E5, E6.} Archived CRISPR and drug-perturbation data, canonical metadata, generated models, execution traces, and prediction metrics. & \textbf{V3 [B,S,R,X].} Evaluated across heterogeneous perturbation datasets, unseen tasks, execution robustness, and expert-designed baselines; no prospective wet-lab testing is reported. \\ \rowcolor{flowDiscovery} scAgents \cite{tang2025scagents} & Single-cell perturbation-model design & \textbf{F1, F2, F3, F4, F5.} Retrieves evidence, designs perturbation models, generates executable code, and evaluates predicted responses. & \textbf{E1, E2, E3, E4, E5, E6.} Literature, archived multimodal perturbation data, persistent knowledge, generated models, executable code, and prediction outputs. & \textbf{V3 [B,S,R,X].} Evaluated across multiple modalities against specialized predictive baselines; validation remains retrospective and in silico. \\ \rowcolor{flowDiscovery} M3A \cite{johri2026evaluating} & Agentic single-cell multiome discovery & \textbf{F1, F2, F4, F5, F6.} Coordinates autonomous and copilot multiomic reasoning over persistent states, with step-level telemetry and expert review. & \textbf{E1, E2, E3, E4, E5, E6.} Pan-cancer snRNA/snATAC data, cNMF programs, TCGA cohorts, clinical endpoints, reasoning traces, and ranked hypotheses. & \textbf{V3 [B,H,S,R,X].} Evaluated across pan-cancer tasks using held-out cohorts, workflow telemetry, blinded expert review, and autonomous-versus-copilot comparisons. \\ \hline \end{tabular} \end{table*} % ============================================================ % Table 9: Interactive and autonomous discovery % ============================================================ 
\begin{table*}[!t] \centering \footnotesize \caption{\textbf{Single-cell and spatial-omics agents: interactive and autonomous discovery.}} \label{tab:single_cell_agents_discovery} \setlength{\tabcolsep}{2pt} \renewcommand{\arraystretch}{1.22} \begin{tabular}{ p{0.10\linewidth} p{0.12\linewidth} p{0.24\linewidth} p{0.24\linewidth} p{0.24\linewidth} } \hline \rowcolor{tableHeader} \textbf{System} & \textbf{Task} & \textbf{Function profile} & \textbf{Evidence profile} & \textbf{Reported V-stage and qualifiers} \\ \hline \flowlabel{flowDiscoveryLabel} {Interactive and Autonomous Discovery} \rowcolor{flowDiscovery} ELISA \cite{coser2026elisa} & Expression-grounded interactive discovery & \textbf{F1, F3, F4.} Routes natural-language queries to expression retrieval, pathway scoring, interaction prediction, comparison, visualization, and reporting. & \textbf{E2, E3, E4, E5.} CELLxGENE datasets, expression and semantic embeddings, differential expression, pathways, ligand--receptor pairs, and retrieval outputs. & \textbf{V3 [B,S,R,X].} Evaluated on six datasets and 100 retrieval queries against CellWhisperer, with replication of published findings. \\ \rowcolor{flowDiscovery} CellVoyager \cite{alber2026cellvoyager} & Autonomous scRNA-seq exploration & \textbf{F1, F3, F4, F5.} Generates, executes, critiques, debugs, and replans notebook-based scRNA-seq analyses and hypotheses. & \textbf{E1, E3, E4, E5.} Published study context, scRNA-seq datasets, generated notebooks, code, plots, interpretations, and independent-dataset analyses. & \textbf{V3 [B,H,R,X].} Benchmarked on analyses from 76 publications with expert-reviewed case studies and independent computational validation; no prospective wet-lab testing is reported. \\ \hline \end{tabular} \end{table*} % ============================================================ % Table 10: Knowledge-grounded discovery % ============================================================ 
\begin{table*}[!t] \centering \footnotesize \caption{\textbf{Single-cell and spatial-omics agents: knowledge-grounded discovery and hypothesis validation.}} \label{tab:single_cell_agents_knowledge} \setlength{\tabcolsep}{2pt} \renewcommand{\arraystretch}{1.22} \begin{tabular}{ p{0.10\linewidth} p{0.12\linewidth} p{0.24\linewidth} p{0.24\linewidth} p{0.24\linewidth} } \hline \rowcolor{tableHeader} \textbf{System} & \textbf{Task} & \textbf{Function profile} & \textbf{Evidence profile} & \textbf{Reported V-stage and qualifiers} \\ \hline \flowlabel{flowDiscoveryLabel} {Knowledge-Grounded Discovery} \rowcolor{flowDiscovery} BiOmics \cite{Cao2026.01.17.699830} & Knowledge-grounded multi-omics reasoning & \textbf{F1, F2, F3, F4, F5, F6.} Coordinates knowledge retrieval, multi-omics tools, graph reasoning, prediction, verification, and evidence-linked reporting. & \textbf{E1, E2, E3, E4, E5.} A large biomedical knowledge graph, literature, multi-omics datasets, tool outputs, graph paths, predictions, and reports. & \textbf{V3 [B,S,R,X].} Evaluated across retrieval, annotation, variant prioritization, trajectory, drug repurposing, spatial, network, and proteomics tasks. \\ \rowcolor{flowDiscovery} OmniCellAgent \cite{huang2025omnicellagent} & Single-cell discovery and hypothesis generation & \textbf{F1, F2, F3, F4, F5.} Coordinates dataset retrieval, differential analysis, enrichment, KG reasoning, literature review, expert synthesis, and reporting. & \textbf{E1, E2, E3, E4, E5.} CELLxGENE/GEO data, enrichment outputs, PrimeKG subgraphs, literature, statistical analyses, ranked hypotheses, and PDF reports. & \textbf{V2 [R,X].} Executable case studies and persistent state support replay, but evaluation remains limited and does not establish broad V3 scientific assessment. \\ \rowcolor{flowDiscovery} PhenoGraph \cite{niyakan2025phenograph} & Phenotype-driven spatial discovery & \textbf{F1, F3, F4, F5.} Retrieves phenotype-matched cohorts, adapts Scissor to spatial data, tunes parameters, and interprets phenotype-associated regions. & \textbf{E2, E3, E4, E5, E6.} Visium and TCGA data, clinical phenotypes, spatial regions, DEGs, survival outputs, and PrimeKG subgraphs. & \textbf{V2 [R,X].} End-to-end execution is demonstrated across breast- and pancreatic-cancer case studies; broad benchmarked evaluation is not established. \\ \rowcolor{flowDiscovery} OmicsNavigator \cite{yiyao2025omicsnavigator} & Auditable spatial-omics hypothesis validation & \textbf{F1, F3, F4, F5, F6.} Curates priors, profiles spatial regions, retrieves biomarkers, and validates hypotheses through pre-registered statistics and human audit. & \textbf{E1, E2, E3, E4, E5, E6.} CODEX/IMC data, morphology and protein profiles, clinical severity, verification blueprints, mixed models, FDR outputs, and audit records. & \textbf{V3 [B,H,S,R,X].} Evaluated across kidney and lung datasets using human labels, ablations, semantic retrieval, pre-registered statistics, and clinical severity associations. \\ \hline \end{tabular} \end{table*}

%=========================================================
 
\begin{table*}[!t] \centering \footnotesize \caption{\textbf{Cross-cutting design requirements for single-cell, spatial biology, cell annotation, and spatial-omics agents.} The requirements distinguish workflow Function, inspectable Evidence, and their contribution to use-case-specific Validation.} \label{tab:singlecell_spatial_crosscutting_patterns} \setlength{\tabcolsep}{3pt} \renewcommand{\arraystretch}{1.18} \begin{tabular}{ p{0.18\linewidth} p{0.28\linewidth} p{0.28\linewidth} p{0.2\linewidth} } \hline \rowcolor{tableHeader} \textbf{Workflow requirement} & \textbf{Domain-specific principle} & \textbf{Inspectable evidence and artifacts} & \textbf{FEV interpretation} \\ \hline % ============================================================ % Requirement 1 % ============================================================ 
\rowcolor{flowAccess} Dataset and context grounding & Identify the assay, samples, tissue, species, condition, cohort, metadata, and analytical objective before selecting tools. & AnnData or Seurat objects, expression matrices, GEO/GSM accessions, sample annotations, tissue labels, disease states, assay metadata, and study context. & \textbf{F1; E3.} Grounded inputs support workflow formulation but do not independently establish replayability. \\ % ============================================================ % Requirement 2 % ============================================================ 
\rowcolor{flowAccess} Cell and spatial representation & Represent cells and regions through expression states, markers, clusters, coordinates, neighborhoods, tissue domains, and perturbation contexts. & Marker tables, UMAPs, cell labels, spatial coordinates, neighborhood graphs, ROI annotations, tissue domains, and multimodal cell profiles. & \textbf{E3; E5} when learned representations are used. Representation quality requires separate evaluation. \\ % ============================================================ % Requirement 3 % ============================================================ 
\rowcolor{flowExecution} Single-cell and spatial tool execution & Execute preprocessing, integration, clustering, annotation, trajectory, interaction, registration, segmentation, and spatial-analysis workflows. & Scanpy, Seurat, CellTypist, scVelo, CellChat, LIANA, Squidpy, MCMICRO, commands, parameters, logs, notebooks, and intermediate outputs. & \textbf{F3; E4.} Execution supports V1; V2 additionally requires replayable environments, parameters, inputs, and traces. \\ % ============================================================ % Requirement 4 % ============================================================ 
\rowcolor{flowEvidence} Annotation and uncertainty assessment & Validate cell-type and tissue-region labels using marker support, confidence, spatial coherence, consensus reasoning, and expert review. & Marker evidence, annotation scores, confidence estimates, heterogeneity flags, consensus labels, spatial-coherence metrics, and reviewer records. & \textbf{F5; F6; E4; E5.} Annotation quality must be established through benchmarks, diagnostics, or expert assessment. \\ % ============================================================ % Requirement 5 % ============================================================ 
\rowcolor{flowEvidence} Biological evidence grounding & Link annotations, trajectories, interactions, and spatial patterns to reference atlases, marker databases, pathways, and literature. & CellMarker, PanglaoDB, CELLxGENE, Cell Ontology, PubMed, GO, Reactome, ligand--receptor resources, retrieved passages, and evidence-linked reports. & \textbf{E1; E2.} Biological sources support attribution but do not independently establish Validation. \\ % ============================================================ % Requirement 6 % ============================================================ 
\rowcolor{flowEvidence} Workflow state, critique, and repair & Preserve analysis state, detect failed tools or implausible outputs, revise plans, repair code, and rerun affected analyses. & Planner and executor traces, failed calls, corrected code, revised notebooks, critic outputs, memory records, repair logs, and workflow histories. & \textbf{F4; F5.} State and repair records support inspection and replay when the complete workflow is reconstructable. \\ % ============================================================ % Requirement 7 % ============================================================ 
\rowcolor{flowEvidence} Provenance-preserving reporting & Report the complete trajectory from molecular inputs to annotations, spatial findings, biological interpretations, and limitations. & Executed code, notebooks, dataset identifiers, parameters, plots, UMAPs, spatial maps, HTML reports, intermediate artifacts, evidence links, uncertainty, and limitations. & \textbf{F4; F6; E4.} Provenance supports replay, audit, and expert review but is not itself a scientific Validation result. \\ % ============================================================ % Requirement 8 % ============================================================ 
\rowcolor{flowClosure} Prospective biological validation & Where required, test an agent-generated annotation, trajectory, interaction, perturbation response, spatial pattern, or biological hypothesis. & Prospective perturbation assays, imaging validation, lineage tracing, targeted marker measurements, functional readouts, and design-linked experimental records. & \textbf{E6; P.} V4 also requires the lower cumulative gates; \textbf{C} requires the new readout to change a subsequent workflow action. \\ \hline \end{tabular} \vspace{0.3em} \begin{minipage}{0.98\textwidth} \footnotesize \textit{Note.} Requirements 1--5 describe the core analytical trajectory summarized in Figure~\ref{fig:singlecell_spatial_crosscutting_fev_blueprint}. Requirements 6--7 operate across that trajectory. Requirement 8 is optional and claim-dependent. Archived perturbation, clinical, or spatial observations contribute to Evidence but not to prospective Validation unless an output of the evaluated workflow is directly tested. \end{minipage} \end{table*}

 \begin{figure*}[!t] \centering \resizebox{0.92\textwidth}{!}{% 
 \begin{tikzpicture}[ x=4.45cm, y=1.0cm, core/.style={ rectangle, rounded corners, draw=blue!65!black, thick, fill=blue!7, text width=3.55cm, minimum height=1.30cm, align=center, font=\scriptsize }, evidenceband/.style={ rectangle, rounded corners, draw=green!55!black, thick, fill=green!7, text width=12.35cm, minimum height=0.92cm, align=center, font=\scriptsize }, control/.style={ rectangle, rounded corners, draw=orange!70!black, thick, fill=orange!8, text width=12.35cm, minimum height=0.88cm, align=center, font=\scriptsize }, empirical/.style={ rectangle, rounded corners, draw=red!65!black, thick, dashed, fill=red!5, text width=8.40cm, minimum height=0.96cm, align=center, font=\scriptsize }, sectionlabel/.style={ anchor=east, text width=1.95cm, align=right, font=\bfseries\scriptsize }, arrow/.style={ -{Latex[length=2mm]}, thick } ] % ============================================================ % Requirements 1--3: data grounding and execution % ============================================================ 
 \node[core] (grounding) at (0,0) { \textbf{1. Dataset and context grounding}\\[0.18em] Resolve assays, samples, tissues, species, conditions, cohorts, metadata, and analytical goals }; \node[core] (representation) at (1,0) { \textbf{2. Cell and spatial representation}\\[0.18em] Represent expression states, markers, clusters, coordinates, neighborhoods, and tissue domains }; \node[core] (execution) at (2,0) { \textbf{3. Single-cell and spatial tool execution}\\[0.18em] Run preprocessing, integration, clustering, annotation, trajectory, interaction, and spatial analysis }; \draw[arrow] (grounding) -- (representation); \draw[arrow] (representation) -- (execution); \node[ sectionlabel, text=blue!65!black ] at ([xshift=-0.35cm]grounding.west) {Data grounding\\and execution}; % ============================================================ % Requirements 4--5: analytical interpretation % Snake layout: % 1 -> 2 -> 3 % | % 5 <- 4 % ============================================================
 \node[core] (evidence) at (0,-2.20) { \textbf{5. Biological evidence grounding}\\[0.18em] Link annotations, trajectories, interactions, and spatial patterns to traceable biological sources }; \node[core] (annotation) at (1,-2.20) { \textbf{4. Annotation and uncertainty assessment}\\[0.18em] Check marker support, confidence, heterogeneity, spatial coherence, consensus, and expert review }; % Empty alignment node used only to preserve the three-column structure 
 \node[ minimum width=3.55cm, minimum height=1.30cm ] (alignment) at (2,-2.20) {}; \draw[arrow] (execution.south) to[out=-90,in=0] (annotation.east); \draw[arrow] (annotation) -- (evidence); \node[ sectionlabel, text=blue!65!black ] at ([xshift=-0.35cm]evidence.west) {Interpretation\\and assessment}; % ============================================================ % Shared evidence and artifacts % ============================================================ 
 \node[evidenceband] (artifacts) at (1,-4.00) { \textbf{Shared single-cell and spatial evidence and artifacts:} AnnData and Seurat objects, expression matrices, marker tables, UMAPs, spatial coordinates, neighborhood graphs, ROI annotations, tool outputs, annotation scores, pathway results, notebooks, plots, and evidence-linked reports }; \node[ sectionlabel, text=green!45!black ] at ([xshift=-0.35cm]artifacts.west) {Shared evidence\\and artifacts}; % ============================================================ % Requirements 6--7: cross-cutting controls % ============================================================ 
 \node[control] (repair) at (1,-5.45) { \textbf{6. Workflow state, critique, and repair:} preserve analytical state, inspect failed calls and implausible outputs, revise plans, repair code, rerun affected steps, and record workflow history }; \node[control] (reporting) at (1,-6.67) { \textbf{7. Provenance-preserving reporting:} retain dataset identifiers, parameters, code, notebooks, intermediate artifacts, spatial maps, evidence links, uncertainty, review records, and limitations }; \node[ sectionlabel, text=orange!70!black ] at ([xshift=-0.35cm]repair.west) {Cross-cutting across\\requirements 1--5}; % ============================================================ % Requirement 8: optional prospective validation % ============================================================ 
 \node[empirical] (validation) at (1,-8.30) { \textbf{8. Optional prospective biological validation}\\[0.15em] Test an agent-generated annotation, trajectory, interaction, perturbation response, spatial pattern, or biological hypothesis. Closed-loop refinement requires the result to change a subsequent action }; \node[ sectionlabel, text=red!65!black ] at ([xshift=-0.35cm]validation.west) {Optional empirical\\extension}; % ============================================================ % Background groupings % ============================================================ 
 \begin{pgfonlayer}{background} \node[ rectangle, rounded corners, draw=blue!22, fill=blue!1, fit=(grounding)(representation)(execution), inner sep=0.15cm ] {}; \node[ rectangle, rounded corners, draw=blue!22, fill=blue!1, fit=(evidence)(annotation), inner sep=0.15cm ] {}; \node[ rectangle, rounded corners, draw=orange!25, fill=orange!1, fit=(repair)(reporting), inner sep=0.16cm ] {}; \end{pgfonlayer} \end{tikzpicture}% 
 } 
 \vspace{-0.2em} \caption{\textbf{Cross-cutting workflow blueprint for single-cell, spatial biology, cell annotation, and spatial-omics agents.} The core trajectory connects dataset and context grounding with cell-level and spatial representation, domain-tool execution, uncertainty-aware annotation, and evidence-linked biological interpretation. Shared artifacts include expression objects, marker tables, spatial coordinates, neighborhood graphs, annotation scores, analytical outputs, and reports. Workflow-state maintenance, repair, and provenance-preserving reporting operate across the trajectory. Prospective biological validation is optional. It constitutes closed-loop refinement only when the resulting empirical evidence changes a subsequent workflow action.} \label{fig:singlecell_spatial_crosscutting_fev_blueprint} \end{figure*}

\subsection{Proteomics, Structural Biology, and Protein-Design Agents} 

Tables~\ref{tab:protein_agents_access}--\ref{tab:protein_agents_empirical} map systems spanning proteomics exploration, evidence-grounded protein interpretation, molecular modelling, protein-engineering workflow execution, de novo sequence design, binder optimization, and experimentally evaluated nanobody or enzyme discovery. Representative tasks include protein-database retrieval, functional-proteomics analysis, Gene Ontology prediction, structure prediction, docking, molecular simulation, sequence redesign, developability filtering, and functional assay validation. The mapped systems range from interactive retrieval platforms to stateful design agents and experimentally connected protein-engineering workflows. 

Despite this diversity, the systems share several recurring workflow requirements, summarized in Figure~\ref{fig:protein_structure_design_crosscutting_fev_blueprint}. Protein objectives must first be translated into explicit sequence, structure, binding, function, stability, or proteomics tasks. Proteins and candidate designs must then be represented through identifiable sequences, structures, domains, complexes, assay measurements, and design constraints. Domain tools are subsequently executed for structure prediction, docking, sequence design, simulation, scoring, visualization, and candidate filtering. Resulting claims should remain linked to protein records, structural models, physical scores, proteomics measurements, literature, and mechanistic evidence. 

Workflow-state maintenance, design critique, quality control, candidate filtering, repair, expert review, and provenance-preserving reporting operate across these activities rather than as isolated final steps. Their importance increases for functional or translational claims, where errors in sequence identity, structure preparation, binding-site selection, scoring, conserved residues, developability assessment, or assay interpretation can propagate into unsupported candidate prioritization. Archived assay measurements contribute to the Evidence profile but do not establish prospective Validation unless an output generated by the evaluated workflow is directly tested. 

Table~\ref{tab:protein_structure_design_crosscutting_patterns} translates these recurring patterns into domain-specific design requirements. It identifies the protein sequences, structures, proteomics measurements, tool calls, simulation outputs, candidate rankings, design traces, and experimental readouts that should remain inspectable. Together, the system maps, synthesis figure, and design-requirement table separate workflow functionality, evidentiary traceability, and use-case-specific validation.

% ============================================================ % Table 12: Protein access, proteomics, and interpretation % ============================================================ 

\begin{table*}[!t] \centering \footnotesize \caption{\textbf{Proteomics, structural-biology, and protein-design agents: protein access, proteomics analysis, and evidence-grounded interpretation.}} \label{tab:protein_agents_access} \setlength{\tabcolsep}{2pt} \renewcommand{\arraystretch}{1.22} \begin{tabular}{ p{0.10\linewidth} p{0.12\linewidth} p{0.24\linewidth} p{0.24\linewidth} p{0.24\linewidth} } \hline \rowcolor{tableHeader} \textbf{System} & \textbf{Task} & \textbf{Function profile} & \textbf{Evidence profile} & \textbf{Reported V-stage and qualifiers} \\ \hline \flowlabel{flowAccessLabel} {Protein Access and Proteomics Exploration} \rowcolor{flowAccess} TourSynbio-Search \cite{liu2024toursynbio} & Protein information retrieval and structure access & \textbf{F1, F3.} Interprets protein-engineering queries, routes them to literature or protein-database search, refines parameters, and retrieves structures. & \textbf{E1, E2, E4.} Retrieved papers, UniProt and PDB records, search parameters, PDB files, and PyMOL visualizations. & \textbf{V1.} Literature and protein-database retrieval with structure visualization is demonstrated, but replayable workflow artifacts and systematic scientific evaluation are not established. \\ \rowcolor{flowAccess} DrBioRight 2.0 \cite{liu2025drbioright} & Cancer functional proteomics exploration & \textbf{F1, F3, F5.} Translates proteomics questions into statistical analyses, visualizations, generated or corrected code, and reports. & \textbf{E2, E3, E4.} RPPA, TCGA and CCLE data, antibody annotations, pathway resources, statistical outputs, generated code, plots, and reports. & \textbf{V1 [H].} Protein-centric cancer analyses and curated expert-facing functionality are demonstrated, but complete workflow replay and systematic evaluation are not established. \\ \flowlabel{flowEvidenceLabel} {Evidence-Grounded Protein Interpretation} \rowcolor{flowEvidence} BioInsight \cite{wang2026bioinsight} & Disease-centred protein interpretation & \textbf{F1, F2, F3, F4, F5, F6.} Coordinates pathway analysis, literature retrieval, protein-level reasoning, citation checking, evidence synthesis, and dashboard generation. & \textbf{E1, E2, E3, E4.} Protein tables, cohort metadata, pathway enrichment, literature, UniProt, STRING, Open Targets, ranked results, evidence packets, and dashboards. & \textbf{V3 [B,H,R].} Replayable analytical artifacts are evaluated on BioASQ, BioInsight-100, and end-to-end disease-level synthesis, with expert assessment of coverage, validity, traceability, prioritization, and usability. \\ \rowcolor{flowEvidence} GOAgent (Zhapa-Camacho et al.) \cite{zhapacamacho2026goagent} & Evidence-grounded protein-function prediction & \textbf{F1, F3, F5, F6.} Uses protein evidence and specialized tools to inspect, verify, and revise Gene Ontology predictions with rationales. & \textbf{E1, E2, E3, E4, E5.} Protein sequences, UniProtKB, PubMed, InterPro, GO constraints, homology outputs, model predictions, revised scores, and rationales. & \textbf{V3 [B,S,R,X].} Evaluated on temporally separated SwissProt data across three GO sub-ontologies using multiple baselines, four metrics, repeated runs, and evidence-source ablations. Predictions remain computational. \\ \rowcolor{flowEvidence} PROTEUS \cite{ding2024automating} & Automated proteomics analysis and hypothesis generation & \textbf{F1, F3, F4, F5, F6.} Plans proteomics analyses, executes specialist tools, interprets intermediate results, revises objectives, and generates testable hypotheses. & \textbf{E1, E2, E3, E4, E5, E6.} CyTOF and mass-spectrometry data, clinical metadata, proteomics tools, statistical outputs, biological hypotheses, and retrospective clinical observations. & \textbf{V3 [B,H,R,X].} Evaluated across 12 proteomics datasets and 191 generated hypotheses using workflow-level assessment and expert review of reliability, coherence, novelty, biological significance, and testability. \\ \flowlabel{flowExecutionLabel} {Molecular Modelling and Tool Execution} \rowcolor{flowExecution} ChatMol Copilot \cite{sun2024chatmol} & Protein and small-molecule computation & \textbf{F1, F3, F4.} Invokes molecular microservices, generates code, maintains cached molecular objects, and visualizes protein or ligand results. & \textbf{E2, E3, E4, E5.} Protein and ligand structures, database records, predicted structures, docking outputs, designed sequences, generated code, and visualizations. & \textbf{V2.} Multi-step molecular workflows, tool calls, cached state, and generated code support replay of reported use cases. Broad scientific benchmarking and prospective testing are not established. \\ \hline \end{tabular} \end{table*} % ============================================================ % Table 13: Executable protein-engineering workflows % ============================================================ 

\begin{table*}[!t] \centering \footnotesize \caption{\textbf{Proteomics, structural-biology, and protein-design agents: executable protein-analysis and engineering workflows.}} \label{tab:protein_agents_execution} \setlength{\tabcolsep}{2pt} \renewcommand{\arraystretch}{1.22} \begin{tabular}{ p{0.10\linewidth} p{0.12\linewidth} p{0.24\linewidth} p{0.24\linewidth} p{0.24\linewidth} } \hline \rowcolor{tableHeader} \textbf{System} & \textbf{Task} & \textbf{Function profile} & \textbf{Evidence profile} & \textbf{Reported V-stage and qualifiers} \\ \hline \flowlabel{flowExecutionLabel} {Executable Protein-Analysis and Engineering Workflows} \rowcolor{flowExecution} AutoProteinEngine (AutoPE) \cite{liu2025autoproteinengine} & Protein-engineering AutoML & \textbf{F1, F3, F4, F5.} Validates task scope, retrieves protein data, configures multimodal models, optimizes hyperparameters, executes training, and summarizes results. & \textbf{E1, E2, E3, E4, E5.} Protein sequences and structures, PDB and UniProt records, model outputs, optimization traces, performance metrics, and generated summaries. & \textbf{V3 [B,S,R].} Evaluated on sweetness classification and enzyme-activity regression against zero-shot and manually tuned baselines, with automated hyperparameter optimization and task-specific predictive metrics. \\ 
\rowcolor{flowExecution} GOAgent (Ponnapati et al.) \cite{ponnapati2026goagent} & Tool-orchestrated protein-function annotation & \textbf{F1, F3, F4, F5.} Orchestrates sequence, structure, and GO tools; maintains multi-turn execution trajectories; and produces sequence- or domain-level annotations with auditable rationales. & \textbf{E2, E3, E4, E5.} Protein sequences, structure-derived features, motif, topology, signal-peptide, binding-site, and Rosetta outputs, GO relations, tool traces, predicted terms, and rationales. & \textbf{V3 [B,S,R,X].} Evaluated on CAFA5 and temporal holdouts against zero-shot, tool-using, trained-agent, and multimodal baselines, with repeated rollouts, bootstrap confidence intervals, tool ablations, and sandbox-execution tests. Predictions remain computational. \\
\rowcolor{flowExecution} AutoBinder Agent \cite{ge2026autobinder} & End-to-end protein-binder design & \textbf{F1, F3, F4, F5.} Plans and executes target analysis, site prediction, seed matching, fragment grafting, sequence redesign, structure prediction, and error recovery through MCP tools. & \textbf{E2, E3, E4, E5.} Target structures, MaSIF outputs, Rosetta grafts, ProteinMPNN sequences, AlphaFold3 complexes, execution logs, and predicted design metrics. & \textbf{V2 [B,R].} A reproducible MCP workflow is evaluated on five standardized behavioural tasks covering planning, tool selection, parameter parsing, recovery, and design execution. Binder quality is not prospectively tested. \\ \rowcolor{flowExecution} PRIME \cite{zhou2025prime} & Dynamic protein-engineering orchestration & \textbf{F1, F2, F3, F4, F5, F6.} Plans DAG-based workflows, selects tools, validates inputs and outputs, recovers from failures, and executes design or model-training tasks. & \textbf{E2, E3, E4, E5.} Protein databases, more than 65 computational tools, workflow DAGs, execution traces, predicted structures, model outputs, and candidate designs. & \textbf{V3 [B,R].} Evaluated on 213 multi-step tasks using completion, tool-use, robustness, and hallucination measures, with additional protein-classification and antibody- design case studies. \\ \rowcolor{flowExecution} ProteinMCP \cite{xu2026proteinmcp} & MCP-based protein-engineering automation & \textbf{F1, F3, F4, F5.} Wraps protein software as reusable MCP tools and executes fitness modelling, binder design, and nanobody-engineering workflows. & \textbf{E2, E3, E4, E5.} MCP tool definitions, sequence and structure inputs, generated models, binder candidates, structural scores, interaction metrics, and execution artifacts. & \textbf{V2 [B,R].} Reusable tool servers and end-to-end case studies support replay of fitness, binder, and nanobody workflows. Candidate quality remains computational and lacks prospective empirical testing. \\ \rowcolor{flowExecution} ProtAgents \cite{ghafarollahi2024protagents} & Protein design and mechanics analysis & \textbf{F1, F2, F3, F5.} Coordinates knowledge retrieval, structure analysis, physics-based simulation, critique, and interpretation for de novo protein design. & \textbf{E1, E2, E3, E4, E5.} Protein sequences, retrieved literature, predicted structures, secondary structures, mechanical predictions, simulations, and tool outputs. & \textbf{V2.} Executable in-silico design and mechanics workflows are demonstrated with inspectable computational outputs. Broad standardized evaluation and prospective wet-lab testing are not established. \\

\hline \end{tabular} \end{table*} % ============================================================ % Table 14: Computational protein design and discovery % ============================================================ 

\begin{table*}[!t] \centering \footnotesize \caption{\textbf{Proteomics, structural-biology, and protein-design agents: computational protein design and discovery.}} \label{tab:protein_agents_design} \setlength{\tabcolsep}{2pt} \renewcommand{\arraystretch}{1.22} \begin{tabular}{ p{0.10\linewidth} p{0.12\linewidth} p{0.24\linewidth} p{0.24\linewidth} p{0.24\linewidth} } \hline \rowcolor{tableHeader} \textbf{System} & \textbf{Task} & \textbf{Function profile} & \textbf{Evidence profile} & \textbf{Reported V-stage and qualifiers} \\ \hline \flowlabel{flowDiscoveryLabel} {Computational Protein Design and Discovery} \rowcolor{flowDiscovery} SPARKS \cite{ghafarollahi2025sparks} & Discovery of protein-design principles & \textbf{F1, F2, F3, F4, F5.} Generates hypotheses, designs computational experiments, executes simulations, refines hypotheses, and produces plots and manuscript-style reports. & \textbf{E1, E3, E4, E5.} Generated sequences, predicted structures, secondary-structure annotations, force and energy predictions, molecular-dynamics traces, plots, and reports. & \textbf{V3 [S,R].} Replayable simulations, quality checks, statistical analyses, and iterative computational experiments support evaluation of generated protein-mechanics hypotheses. Prospective wet-lab validation is not reported. \\ \rowcolor{flowDiscovery} PDAgent \cite{ouyangpdagent} & Conservation-aware protein redesign & \textbf{F1, F3, F4, F5.} Translates property requirements into design constraints, retrieves templates, protects conserved residues, proposes mutations, scores candidates, and iteratively revises sequences. & \textbf{E2, E3, E4, E5.} UniProt templates, homologous sequences, multiple-sequence alignments, conservation scores, stability filters, predicted structures, and design histories. & \textbf{V3 [B,S,R].} Evaluated across 100 design tasks using generation success, foldability, constraint satisfaction, model comparisons, and ablations of iterative reasoning components. \\ \rowcolor{flowDiscovery} VibeGen \cite{ni2026vibegen} & Dynamics-conditioned protein design & \textit{Agent-adjacent generative--predictive loop;} \textbf{F3, F5.} Executes structural and dynamics evaluation within a coupled design loop and revises candidates using predictive feedback. & \textbf{E3, E4, E5.} Target dynamics, generated sequences, predicted structures, simulations, and dynamic-accuracy metrics. & \textbf{V3 [B].} Evaluated on 1,293 held-out proteins using structural, dynamic, diversity, and novelty analyses; validation remains computational. \\
\rowcolor{flowDiscovery} ProteinCrow \cite{ponnapati2025proteincrow} & Protein redesign and binder optimization & \textbf{F1, F3, F4, F5.} Plans and executes stability optimization, functional-site-preserving redesign, binder generation, sequence filtering, and deimmunization. & \textbf{E1, E2, E3, E4, E5.} Literature, UniProt records, protein structures, design-model outputs, Rosetta scores, structural-confidence measures, epitope predictions, and ranked candidates. & \textbf{V3 [B,R].} Evaluated across stability, constrained redesign, binder generation, and epitope-reduction tasks using computational baselines, structural checks, design filters, and tool-trajectory analyses. \\ \rowcolor{flowDiscovery} AgentPLM \cite{rahman2026agentplm} & Tool-guided protein-sequence design & \textit{Model-level tool-using agent;} \textbf{F3, F4, F5.} Interleaves sequence generation with biophysical tool calls, retains trajectory memory, and redirects decoding using structural, stability, and binding feedback. & \textbf{E2, E3, E4, E5.} Protein datasets, generated sequences, ESMFold, FoldX and Vina outputs, fitness predictions, and trajectory records. & \textbf{V3 [B,R].} Evaluated across five protein-design settings against passive and tool-augmented baselines, with ablations and trajectory analyses; validation remains in silico. \\ \hline \end{tabular} \end{table*} % ============================================================ % Table 15: Prospective experimental validation % ============================================================ 

\begin{table*}[!t] \centering \footnotesize \caption{\textbf{Proteomics, structural-biology, and protein-design agents: prospective experimental evaluation.}} \label{tab:protein_agents_empirical} \setlength{\tabcolsep}{2pt} \renewcommand{\arraystretch}{1.22} \begin{tabular}{ p{0.10\linewidth} p{0.12\linewidth} p{0.24\linewidth} p{0.24\linewidth} p{0.24\linewidth} } \hline \rowcolor{tableHeader} \textbf{System} & \textbf{Task} & \textbf{Function profile} & \textbf{Evidence profile} & \textbf{Reported V-stage and qualifiers} \\ \hline \flowlabel{flowClosureLabel} {Prospective Functional Evaluation} \rowcolor{flowClosure} ProteinSwarm / Swarms of LLM Agents \cite{wang2025swarms} & Swarm-based protein-sequence design & \textbf{F1, F2, F3, F4, F5.} Coordinates residue-specific agents that propose, score, remember, and revise mutations using local structural context and design objectives. & \textbf{E3, E4, E5, E6.} Generated sequences, predicted structures, Rosetta energies, secondary- structure outputs, design histories, and prospective circular-dichroism measurements. & \textbf{V4 [B,R,P].} Computational design is combined with prospective circular-dichroism testing of two agent-generated peptides. The assays validate intended helix and coil structures, although complete protein function and binding remain untested. \\ \rowcolor{flowClosure} Agent-Guided Cancer Nanobody Design \cite{zhao2026agent} & De novo nanobody design against a cancer target & \textbf{F1, F3, F4, F5, F6.} Identifies epitope hotspots, generates and scores VHH candidates, applies developability filters, performs Pareto selection, and prioritizes candidates for binding assays. & \textbf{E2, E3, E4, E5, E6.} Target sequences and predicted structures, nanobody designs, structural and binding scores, liability profiles, yeast-display results, FACS enrichment, and SPR kinetics. & \textbf{V4 [B,S,R,P].} Agent-guided candidates are prospectively evaluated by yeast surface display, FACS, and SPR, yielding experimentally confirmed binders with nanomolar to sub-nanomolar affinities. Epitope and cell-based validation remain future work. \\ \rowcolor{flowClosure} Virtual Lab \cite{swanson2025virtual} & AI--human nanobody discovery & \textbf{F1, F2, F3, F4, F5, F6.} Coordinates principal-investigator, specialist, and critic agents to design pipelines, evaluate structures, prioritize nanobodies, and support experimental testing. & \textbf{E1, E2, E3, E4, E5, E6.} Literature, designed sequences, ESM and AlphaFold-Multimer outputs, Rosetta scores, expression and solubility results, antigen-array binding, and ELISA measurements. & \textbf{V4 [B,H,P].} Computationally prioritized nanobody candidates are prospectively tested through expression, solubility, antigen-array, and ELISA assays in an AI--human scientific workflow. \\ \rowcolor{flowClosure} ORI \cite{he2026functional} & Closed-loop protein engineering & \textit{Agent-adjacent model--laboratory framework;} \textbf{F3, F4, F5.} Generates and filters proteins, preserves iterative design state, and updates optimization using wet-lab feedback. & \textbf{E2, E3, E4, E5, E6.} Ontology constraints, generated proteins, model outputs, quality checks, functional assays, and feedback records. & \textbf{V4 [B,P,C].} Generated proteins undergo prospective functional testing, and assay outcomes update subsequent reinforcement-based optimization. \\
\hline \end{tabular} \vspace{0.3em} \begin{minipage}{0.98\textwidth} \footnotesize \textit{Note.} Prospective empirical testing of an agent-generated protein or peptide contributes qualifier P. Qualifier C is assigned only when the resulting experimental measurement changes a subsequent design or optimization action. The scope of V4 remains claim-specific: structural validation of a peptide does not establish protein function, binding, developability, or therapeutic utility. \end{minipage} \end{table*}

\begin{table*}[!t] \centering \footnotesize \caption{\textbf{Cross-cutting design requirements for proteomics, structural biology, and protein-design agents.} The requirements distinguish workflow Function, inspectable Evidence, and their contribution to use-case-specific Validation.} \label{tab:protein_structure_design_crosscutting_patterns} \setlength{\tabcolsep}{3pt} \renewcommand{\arraystretch}{1.18} \begin{tabular}{ p{0.18\linewidth} p{0.28\linewidth} p{0.28\linewidth} p{0.2\linewidth} } \hline \rowcolor{tableHeader} \textbf{Workflow requirement} & \textbf{Domain-specific principle} & \textbf{Inspectable evidence and artifacts} & \textbf{FEV interpretation} \\ \hline % ============================================================ % Requirement 1 % ============================================================ 
\rowcolor{flowAccess} Protein objective and constraints & Define the proteomics, structural-analysis, docking, sequence-design, simulation, or candidate-prioritization objective and its design constraints. & Research question, target protein, desired function, binding site, sequence constraints, assay requirements, design objectives, and candidate-selection criteria. & \textbf{F1.} Objective formulation defines the workflow but does not establish execution or scientific validity. \\ % ============================================================ % Requirement 2 % ============================================================ 
\rowcolor{flowAccess} Protein and proteomics data grounding & Resolve protein identities, sequences, structures, domains, complexes, proteomics measurements, ligands, templates, and candidate designs. & UniProt identifiers, FASTA sequences, PDB structures, AlphaFold models, RPPA or mass-spectrometry data, antibody panels, ligand structures, multiple-sequence alignments, and assay metadata. & \textbf{E2; E3.} Traceable molecular inputs are necessary, but not sufficient, for replayability. \\ % ============================================================ % Requirement 3 % ============================================================ 
\rowcolor{flowExecution} Molecular tool execution & Execute structure prediction, sequence design, docking, simulation, visualization, proteomics analysis, and candidate-scoring workflows. & Tool calls, parameters, versions, logs, generated code, intermediate files, and outputs from AlphaFold, ESMFold, ProteinMPNN, RFdiffusion, Rosetta, AutoDock Vina, RDKit, and related tools. & \textbf{F3; E4.} Execution supports V1; V2 additionally requires replayable inputs, environments, parameters, and traces. \\ % ============================================================ % Requirement 4 % ============================================================ 
\rowcolor{flowExecution} Structural and functional evaluation & Assess candidate structures, interfaces, dynamics, stability, binding, developability, and predicted biological function. & Predicted structures, pLDDT and ipTM scores, docking poses, binding scores, Rosetta energies, molecular-dynamics traces, secondary structures, stability estimates, and developability metrics. & \textbf{E4; E5.} Computational scores support candidate assessment, but scientific adequacy requires benchmark, robustness, or expert evaluation. \\ % ============================================================ % Requirement 5 % ============================================================ 
\rowcolor{flowEvidence} Biological and mechanistic grounding & Connect proteomics results and candidate designs to protein function, pathways, conserved residues, binding mechanisms, disease context, and literature. & PubMed, UniProt, PDB, InterPro, Gene Ontology, pathway resources, homology evidence, conserved sites, protein--protein interactions, mechanistic rationales, and evidence-linked reports. & \textbf{E1; E2.} Biological sources support interpretation and attribution but do not independently establish Validation. \\ % ============================================================ % Requirement 6 % ============================================================ 
\rowcolor{flowEvidence} Design critique, filtering, and repair & Reject implausible candidates, detect failed tools or structural defects, apply functional and developability filters, and revise the design workflow. & Critic outputs, failed calls, repaired code, revised sequences, structure-quality checks, energy thresholds, conservation constraints, liability filters, and ranked candidates. & \textbf{F4; F5; F6.} Critique and filtering are workflow capabilities whose effectiveness must be established through task-appropriate Validation. \\ % ============================================================ % Requirement 7 % ============================================================ 
\rowcolor{flowEvidence} Trace and provenance preservation & Preserve the trajectory from protein inputs and design constraints to tool execution, candidate evaluation, selection, and reporting. & Dataset and structure identifiers, software versions, parameters, scripts, notebooks, JSON records, design histories, intermediate structures, simulation files, molecular visualizations, rankings, and limitations. & \textbf{F4; E4.} Provenance supports replay and audit only when the evaluated workflow can be reconstructed from the reported artifacts. \\ % ============================================================ % Requirement 8 % ============================================================ 
\rowcolor{flowClosure} Prospective functional validation & Test an agent-generated protein, peptide, binder, nanobody, or enzyme using an assay aligned with the principal structural or functional claim. & Expression and solubility measurements, circular dichroism, yeast surface display, FACS, SPR, ELISA, binding assays, enzyme-activity measurements, thermostability assays, and design-linked experimental records. & \textbf{E6; P.} V4 also requires the lower cumulative gates; \textbf{C} requires the experimental result to change a subsequent design action. \\ \hline \end{tabular} \vspace{0.3em} \begin{minipage}{0.98\textwidth} \footnotesize \textit{Note.} Requirements 1--5 define the core workflow summarized in Figure~\ref{fig:protein_structure_design_crosscutting_fev_blueprint}. Requirements 6--7 operate across that workflow. Requirement 8 is optional and claim-dependent. Archived assay measurements contribute to Evidence but not to prospective Validation unless an output generated by the evaluated workflow is directly tested. \end{minipage} \end{table*}

\begin{figure*}[!t] \centering \resizebox{0.92\textwidth}{!}{% 
\begin{tikzpicture}[ x=4.45cm, y=1.0cm, core/.style={ rectangle, rounded corners, draw=blue!65!black, thick, fill=blue!7, text width=3.55cm, minimum height=1.30cm, align=center, font=\scriptsize }, evidenceband/.style={ rectangle, rounded corners, draw=green!55!black, thick, fill=green!7, text width=12.35cm, minimum height=0.92cm, align=center, font=\scriptsize }, control/.style={ rectangle, rounded corners, draw=orange!70!black, thick, fill=orange!8, text width=12.35cm, minimum height=0.88cm, align=center, font=\scriptsize }, empirical/.style={ rectangle, rounded corners, draw=red!65!black, thick, dashed, fill=red!5, text width=8.40cm, minimum height=0.96cm, align=center, font=\scriptsize }, sectionlabel/.style={ anchor=east, text width=1.95cm, align=right, font=\bfseries\scriptsize }, arrow/.style={ -{Latex[length=2mm]}, thick } ] % ============================================================ % Requirements 1--3: objective, grounding, and execution % ============================================================ 
\node[core] (objective) at (0,0) { \textbf{1. Protein objective and constraints}\\[0.18em] Define the proteomics, structure, binding, function, stability, or sequence-design task }; \node[core] (grounding) at (1,0) { \textbf{2. Protein and proteomics data grounding}\\[0.18em] Resolve sequences, structures, domains, complexes, measurements, templates, and candidate designs }; \node[core] (execution) at (2,0) { \textbf{3. Molecular tool execution}\\[0.18em] Run structure prediction, docking, sequence design, simulation, scoring, and visualization }; \draw[arrow] (objective) -- (grounding); \draw[arrow] (grounding) -- (execution); \node[ sectionlabel, text=blue!65!black ] at ([xshift=-0.35cm]objective.west) {Workflow formulation\\and execution}; % ============================================================ % Requirements 4--5: evaluation and interpretation % ============================================================ 
\node[core] (mechanism) at (0,-2.20) { \textbf{5. Biological and mechanistic grounding}\\[0.18em] Link designs and proteomics results to functions, pathways, conserved sites, mechanisms, and literature }; \node[core] (evaluation) at (1,-2.20) { \textbf{4. Structural and functional evaluation}\\[0.18em] Assess structures, interfaces, dynamics, stability, binding, function, and developability }; \node[ minimum width=3.55cm, minimum height=1.30cm ] (alignment) at (2,-2.20) {}; \draw[arrow] (execution.south) to[out=-90,in=0] (evaluation.east); \draw[arrow] (evaluation) -- (mechanism); \node[ sectionlabel, text=blue!65!black ] at ([xshift=-0.35cm]mechanism.west) {Candidate evaluation\\and interpretation}; % ============================================================ % Shared evidence and artifacts % ============================================================ 
\node[evidenceband] (artifacts) at (1,-4.00) { \textbf{Shared protein evidence and artifacts:} FASTA sequences, UniProt and PDB records, proteomics measurements, predicted structures, docking poses, Rosetta energies, molecular-dynamics traces, stability and developability scores, candidate rankings, experimental protocols, and evidence-linked reports }; \node[ sectionlabel, text=green!45!black ] at ([xshift=-0.35cm]artifacts.west) {Shared evidence\\and artifacts}; % ============================================================ % Requirements 6--7: cross-cutting controls % ============================================================ 
\node[control] (critique) at (1,-5.45) { \textbf{6. Design critique, filtering, and repair:} inspect sequence and structure quality, conserved residues, docking or energy scores, failed tools, functional constraints, developability liabilities, and revise weak candidates or workflows }; \node[control] (provenance) at (1,-6.67) { \textbf{7. Trace and provenance preservation:} retain identifiers, design constraints, tool versions, parameters, code, intermediate structures, simulation files, design histories, candidate rankings, expert-review records, and limitations }; \node[ sectionlabel, text=orange!70!black ] at ([xshift=-0.35cm]critique.west) {Cross-cutting across\\requirements 1--5}; % ============================================================ % Requirement 8: optional prospective validation % ============================================================ 
\node[empirical] (validation) at (1,-8.30) { \textbf{8. Optional prospective functional validation}\\[0.15em] Test an agent-generated protein, peptide, binder, nanobody, or enzyme using expression, structural, binding, stability, or functional assays. Closed-loop refinement requires the result to change a subsequent design action }; \node[ sectionlabel, text=red!65!black ] at ([xshift=-0.35cm]validation.west) {Optional empirical\\extension}; % ============================================================ % Background groupings % ============================================================ 
\begin{pgfonlayer}{background} \node[ rectangle, rounded corners, draw=blue!22, fill=blue!1, fit=(objective)(grounding)(execution), inner sep=0.15cm ] {}; \node[ rectangle, rounded corners, draw=blue!22, fill=blue!1, fit=(mechanism)(evaluation), inner sep=0.15cm ] {}; \node[ rectangle, rounded corners, draw=orange!25, fill=orange!1, fit=(critique)(provenance), inner sep=0.16cm ] {}; \end{pgfonlayer} \end{tikzpicture}% 
} \vspace{-0.2em} \caption{\textbf{Cross-cutting workflow blueprint for proteomics, structural biology, and protein-design agents.} The core trajectory connects protein-objective formulation and molecular-data grounding with tool-mediated structure prediction, docking, simulation, sequence design, candidate evaluation, and evidence-linked interpretation. Shared artifacts include protein sequences, structures, proteomics measurements, docking poses, energy scores, simulation outputs, candidate rankings, and reports. Design critique, filtering, repair, and provenance preservation operate across the workflow. Prospective functional validation is optional. It constitutes closed-loop refinement only when the resulting experimental evidence changes a subsequent design action.} \label{fig:protein_structure_design_crosscutting_fev_blueprint} \end{figure*}

\subsection{Drug Discovery, Therapeutic Reasoning, and Molecular Design Agents} 

Tables~\ref{tab:drug_agents_reasoning}-- \ref{tab:drug_agents_clinical} map systems spanning target assessment, drug repurposing, mechanism-of-action reasoning, therapeutic recommendation, predictive modelling, molecular design, pharmacovigilance, and target-trial emulation. Representative tasks include target-dossier generation, drug--disease prioritization, ADMET and drug--target prediction, molecular screening and optimization, adverse-event extraction, clinical-trial outcome prediction, and causal analysis of real-world clinical data. The mapped systems range from evidence-retrieval assistants to stateful agents that execute, evaluate, and revise computational or clinical-analysis workflows. 

Despite this diversity, the systems share several recurring workflow requirements, summarized in Figure~\ref{fig:drug_discovery_crosscutting_fev_blueprint}. Therapeutic objectives must first be translated into explicit target-identification, molecular-design, safety, treatment, or trial-analysis tasks. Drugs, targets, molecules, patients, cohorts, and trials must then be represented through normalized identifiers, structures, indications, endpoints, eligibility criteria, and safety attributes. Domain tools, databases, knowledge graphs, predictive models, docking workflows, and clinical-analysis methods are subsequently executed to generate inspectable computational evidence. Resulting claims should remain linked to molecular structures, target records, mechanistic paths, safety evidence, trial assumptions, statistical outputs, and retrieved biomedical sources. 

Workflow-state maintenance, safety checking, critique, repair, verification, expert review, and provenance preservation operate across these activities rather than as isolated final steps. Their importance increases for patient-specific recommendations, toxicity assessment, clinical-trial reasoning, and therapeutic candidate prioritization, where errors in entity normalization, cohort construction, endpoint definition, causal assumptions, molecular scoring, or evidence attribution can lead to unsupported conclusions. Archived pharmacological, preclinical, or clinical observations contribute to the Evidence profile but do not establish prospective Validation unless an output generated by the evaluated workflow is directly tested. 

Table~\ref{tab:drug_discovery_crosscutting_patterns} translates these recurring patterns into domain-specific design requirements. It identifies the molecular representations, target records, retrieved evidence, model outputs, safety checks, statistical artifacts, workflow traces, and empirical readouts that should remain inspectable. Together, the system maps, synthesis figure, and design-requirement table separate workflow functionality, evidentiary traceability, and use-case-specific validation.

% ============================================================ % Table 17: Target intelligence, therapeutic reasoning, % and predictive modelling % ============================================================ 
\begin{table*}[!t] \centering \footnotesize \caption{\textbf{Drug-discovery, therapeutic-reasoning, and molecular-design agents: target intelligence, evidence-grounded reasoning, and predictive modelling.}} \label{tab:drug_agents_reasoning} \setlength{\tabcolsep}{2pt} \renewcommand{\arraystretch}{1.22} \begin{tabular}{ p{0.10\linewidth} p{0.12\linewidth} p{0.24\linewidth} p{0.24\linewidth} p{0.24\linewidth} } \hline \rowcolor{tableHeader} \textbf{System} & \textbf{Task} & \textbf{Function profile} & \textbf{Evidence profile} & \textbf{Reported V-stage and qualifiers} \\ \hline % ============================================================ % Target intelligence and evidence access % ============================================================ 
\flowlabel{flowAccessLabel} {Target Intelligence and Evidence Access} \rowcolor{flowAccess} SwiftDossier \cite{fossi2024swiftdossier} & Drug-target dossier generation & \textbf{F1, F3, F4, F5.} Plans target assessment, retrieves biomedical evidence, executes sequence and enrichment tools, and compiles traceable target dossiers. & \textbf{E1, E2, E4.} PubMed/PMC, UniProt, Open Targets, DrugBank, PDB, STRING, BLAST, enrichment outputs, citations, and generated PDF or PowerPoint dossiers. & \textbf{V2 [H,R].} Executable retrieval and analysis artifacts support replay of reported dossiers. Expert-facing review and source checks are reported, but broader scientific evaluation remains limited. \\ % ============================================================ % Evidence-grounded therapeutic reasoning % ============================================================ 
\flowlabel{flowEvidenceLabel} {Evidence-Grounded Therapeutic Reasoning} \rowcolor{flowEvidence} BioScientist Agent \cite{zhang2025bioscientist} & Drug repurposing and mechanism-of-action reasoning & \textbf{F1, F2, F3, F4, F5.} Combines drug--disease prediction, graph-path search, causal-literature retrieval, evidence scoring, and mechanistic report generation. & \textbf{E1, E2, E4, E5.} RTX-KG2, DrugBank, ChEMBL, UniProt, DisGeNET, PubMed causal statements, predicted links, ranked mechanism paths, and evidence scores. & \textbf{V3 [B,R].} Evaluated against graph and KG-based baselines for drug-repurposing and mechanism-path ranking, with component analyses. Predictions remain computational hypotheses. \\ \rowcolor{flowEvidence} TCM-Agent \cite{wang2026tcm} & Traditional-medicine network pharmacology & \textbf{F1, F2, F3, F4, F5, F6.} Normalizes herbs, compounds, targets, and diseases; executes network, ADMET, similarity, PPI, and enrichment analyses; and generates evidence-graded reports. & \textbf{E1, E2, E3, E4, E5, E6.} TCM and chemical databases, PubMed, compound--target records, ADMET predictions, PPI and pathway outputs, mechanistic reports, and archived experimental observations. & \textbf{V3 [B,H,R,X].} Evaluated on 100 curated studies and 563 questions using multiple model backbones, expert scoring, workflow comparisons, and a liver-fibrosis case study. Therapeutic claims lack prospective targeted validation. \\ \rowcolor{flowEvidence} TXAGENT \cite{gao2025txagent} & Therapeutic reasoning and treatment recommendation & \textbf{F1, F3, F4, F5, F6.} Selects tools, retrieves current drug evidence, checks interactions and contraindications, and synthesizes patient- or indication-specific recommendations. & \textbf{E1, E2, E4, E5, E6.} FDA labels, openFDA, Open Targets, HPO, PrimeKG, tool outputs, interaction records, treatment predictions, and benchmark cases. & \textbf{V3 [B,R].} Evaluated on large drug-reasoning and treatment benchmarks with explicit tool traces and routing analyses. Prospective clinical deployment and patient-outcome validation are not established. \\ \rowcolor{flowEvidence} CLADD \cite{lee2026rag} & Molecular reasoning and prediction & \textbf{F1, F2, F3, F5.} Coordinates planning, molecular retrieval, knowledge-graph reasoning, molecular interpretation, and predictive agents across zero-shot tasks. & \textbf{E2, E3, E4, E5.} SMILES strings, PubChem annotations, PrimeKG paths, retrieved molecular anchors, generated captions, similarity scores, and molecular predictions. & \textbf{V3 [B,R].} Evaluated across drug--target, molecular-captioning, toxicity, and antibacterial-activity tasks against predictive and language-model baselines. Performance depends on retrieval and anchor coverage. \\ % ============================================================ % Predictive modelling and tool-grounded execution % ============================================================ 
\flowlabel{flowExecutionLabel} {Predictive Modelling and Tool-Grounded Execution} \rowcolor{flowExecution} TxGemma / Agentic-Tx \cite{wang2025txgemma} & Generalist therapeutic prediction and reasoning & \textbf{F1, F3, F4, F5.} Routes therapeutic tasks to predictive models and external knowledge for property, toxicity, pharmacokinetic, interaction, and trial reasoning. & \textbf{E2, E3, E4, E5, E6.} Therapeutics Data Commons, molecular and biological sequences, clinical-trial records, property predictions, adverse-event outputs, and reasoning traces. & \textbf{V3 [B,R,X].} Broadly evaluated across therapeutic prediction, molecular reasoning, and clinical-trial tasks with model and retrieval comparisons. Evaluation remains computational and retrospective. \\ \rowcolor{flowExecution} DrugAgent \cite{liu2024drugagent} & Drug-discovery machine-learning programming & \textbf{F1, F2, F3, F4, F5.} Coordinates solution planning, molecular featurization, model selection, code generation, unit testing, execution, and self-debugging. & \textbf{E2, E3, E4, E5.} ADMET, HTS, and DTI datasets; SMILES and protein sequences; generated training code, molecular descriptors, predictions, and submission files. & \textbf{V3 [B,R].} Evaluated across ADMET, screening, and drug--target tasks against CoT, ReAct, and ResearchAgent, with execution and debugging analyses. Validation remains in silico. \\ \hline \end{tabular} \end{table*} % ============================================================ % Table 18: Tool-grounded execution and molecular design % ============================================================
\begin{table*}[!t] \centering \footnotesize \caption{\textbf{Drug-discovery, therapeutic-reasoning, and molecular-design agents: tool-grounded execution, molecular screening, and lead optimization.}} \label{tab:drug_agents_design} \setlength{\tabcolsep}{2pt} \renewcommand{\arraystretch}{1.22} \begin{tabular}{ p{0.10\linewidth} p{0.12\linewidth} p{0.24\linewidth} p{0.24\linewidth} p{0.24\linewidth} } \hline \rowcolor{tableHeader} \textbf{System} & \textbf{Task} & \textbf{Function profile} & \textbf{Evidence profile} & \textbf{Reported V-stage and qualifiers} \\ \hline % ============================================================ % Predictive modelling and tool-grounded execution % ============================================================ 
\flowlabel{flowExecutionLabel} {Tool-Grounded Molecular Execution} \rowcolor{flowExecution} BioChemAIgent \cite{yousefi2025biochemaigent} & Protein modelling and molecular docking & \textbf{F1, F3, F4, F5, F6.} Coordinates MCP tools for molecular preparation, structure modelling, docking, interaction analysis, visualization, and error handling. & \textbf{E2, E3, E4, E5.} PubChem and PDB records, protein and ligand structures, predicted models, docking poses, interaction outputs, tool logs, and molecular visualizations. & \textbf{V3 [B,H,R].} Evaluated using expert-curated tasks, corrupted-query robustness tests, four realistic expert-reviewed scenarios, and a COX-1 docking case study. Binding and pharmacological activity remain computational. \\ \rowcolor{flowExecution} DrugPilot \cite{li2025drugpilot} & Parameterized drug-discovery tool execution & \textbf{F1, F3, F4, F5.} Maintains structured parameters across turns, invokes predictive and generative tools, corrects invalid calls, and continues multi-step workflows. & \textbf{E2, E3, E4, E5.} TCDD tasks, molecular and pharmacological datasets, structured memory, tool parameters, model predictions, generated molecules, and execution logs. & \textbf{V3 [B,R].} Evaluated on simple, multi-tool, and multi-turn scenarios against ReAct, CoT, and LoT, with ablations of memory, feedback, and fine-tuning components. Evaluation measures computational tool competence. \\ % ============================================================ % Molecular design and optimization % ============================================================ 
\flowlabel{flowDiscoveryLabel} {Molecular Design and Lead Optimization} \rowcolor{flowDiscovery} MolLingo \cite{nguyen2026mollingo} & Molecular design and lead optimization & \textbf{F1, F2, F3, F4, F5.} Coordinates literature and chemistry agents for target identification, hit discovery, fragment growth, docking, and ADMET-aware optimization. & \textbf{E1, E2, E3, E4, E5, E6.} PubMed, UniProt, ChEMBL, molecular structures, docking poses, ADMET predictions, toxicity records, candidate rankings, and shared design memory. & \textbf{V3 [B,S,R,X].} Evaluated across ADMET optimization, docking-guided design, property optimization, and hit discovery against language-model and molecular-design baselines. Generated leads remain computational candidates. \\ \rowcolor{flowDiscovery} MolClaw \cite{zhang2026molclaw} & Hierarchical molecular screening and optimization & \textbf{F1, F3, F4, F5, F6.} Composes validated tool and workflow skills, applies scientific quality gates, recovers from failures, preserves provenance, and executes long-horizon molecular-discovery workflows. & \textbf{E2, E3, E4, E5.} Molecular and protein databases, docking and dynamics outputs, interaction profiles, ADMET predictions, optimized molecules, execution traces, and quality-control records. & \textbf{V3 [B,S,R].} Evaluated on MolBench screening, editing, optimization, and end-to-end tasks, including workflows spanning 8--50 or more steps, with statistical comparison and failure-recovery analyses. \\ \rowcolor{flowDiscovery} PharmAgents \cite{gao2025pharmagents} & Virtual pharmaceutical discovery & \textbf{F1, F2, F3, F4, F5.} Coordinates target discovery, lead generation and optimization, docking, toxicity and metabolism assessment, synthesizability analysis, and experience-based refinement. & \textbf{E2, E3, E4, E5.} Drug and target databases, predicted structures, generated molecules, docking and interaction outputs, toxicity and metabolism predictions, synthesis assessments, reports, and experience memory. & \textbf{V2 [R].} The reported virtual-pharma workflows provide traceable multi-step computational artifacts and iterative refinement. Broad independent scientific evaluation and empirical testing are not established. \\ \rowcolor{flowDiscovery} Mozi \cite{cao2026mozi} & Governed drug-discovery workflow & \textbf{F1, F2, F3, F4, F5, F6.} Uses supervisor--worker control, role-isolated tools, stateful skill graphs, reflection, human checkpoints, and auditable execution across discovery stages. & \textbf{E1, E2, E3, E4, E5.} Biomedical databases, molecular tools, workflow states, docking and DTI scores, toxicity filters, generated candidates, human-review records, and execution traces. & \textbf{V3 [B,H,R].} Evaluated through PharmaBench, governed tool-routing tests, role isolation, error-containment analyses, human checkpoints, and three end-to-end disease case studies. Candidates remain in silico. \\ \hline \end{tabular} \end{table*} % ============================================================ % Table 19: Safety and clinical translation % ============================================================ 
\begin{table*}[!t] \centering \footnotesize \caption{\textbf{Drug-discovery, therapeutic-reasoning, and molecular-design agents: safety analysis and clinical translation.}} \label{tab:drug_agents_clinical} \setlength{\tabcolsep}{2pt} \renewcommand{\arraystretch}{1.22} \begin{tabular}{ p{0.10\linewidth} p{0.12\linewidth} p{0.24\linewidth} p{0.24\linewidth} p{0.24\linewidth} } \hline \rowcolor{tableHeader} \textbf{System} & \textbf{Task} & \textbf{Function profile} & \textbf{Evidence profile} & \textbf{Reported V-stage and qualifiers} \\ \hline \flowlabel{flowTranslationLabel} {Safety and Clinical Translation} \rowcolor{flowTranslation} MALADE \cite{choi2024malade} & Pharmacovigilance and adverse-event extraction & \textbf{F1, F2, F3, F4, F5, F6.} Selects representative drugs, retrieves FDA labels, extracts adverse events, aggregates evidence by drug category, and validates outputs through critics. & \textbf{E1, E2, E3, E4, E6.} FDA drug labels, NDC records, MIMIC-IV prescriptions, OMOP adverse-event references, retrieved passages, confidence estimates, rationales, and critic logs. & \textbf{V3 [B,S,R].} Evaluated against OMOP adverse-event references with structured confidence, rationales, and critic-supported verification. Results depend on label coverage, category mapping, and retrospective ground truth. \\ \rowcolor{flowTranslation} AUTOCT \cite{liu2025autoct} & Clinical-trial outcome prediction & \textbf{F1, F3, F4, F5.} Proposes, retrieves, builds, evaluates, and refines interpretable clinical-trial features through MCTS and classical predictive models. & \textbf{E1, E2, E3, E4, E5, E6.} ClinicalTrials.gov records, PubMed evidence, historical trial outcomes, generated feature schemas, predictive models, SHAP explanations, and ROC-AUC results. & \textbf{V3 [B,S,R].} Evaluated on TrialBench-derived approval, dropout, mortality, and adverse-event tasks using interpretable models and iterative feature refinement. Cohorts are sampled and evaluation remains retrospective. \\ \rowcolor{flowTranslation} EmulatRx \cite{li2026empowering} & Target-trial design and emulation & \textbf{F1, F2, F3, F4, F5, F6.} Coordinates trialist, informatician, clinician, and statistician agents to translate protocols into cohort definitions, SQL, causal analyses, and reviewed trial-emulation reports. & \textbf{E1, E2, E3, E4, E6.} Trial protocols, MIMIC-IV and INSIGHT records, OMOP concepts, generated SQL, propensity scores, IPTW and clone--censor--weight outputs, Cox models, Kaplan--Meier curves, and endpoint analyses. & \textbf{V3 [B,H,S,R,X].} Evaluated on acute and chronic target-trial emulations using protocol, SQL, cohort, and causal-analysis metrics, with clinical and statistical review across multiple health-data settings. Prospective trial-design impact is not established. \\ \hline \end{tabular} \vspace{0.3em} \begin{minipage}{0.98\textwidth} \footnotesize \textit{Note.} Clinical records, trial outcomes, adverse-event observations, and historical pharmacological measurements contribute to the Evidence profile, including E6 where appropriate. They do not constitute prospective Validation unless an output generated by the evaluated workflow is directly tested in a new experimental, preclinical, or clinical setting. \end{minipage} \end{table*}

\begin{table*}[!t] \centering \footnotesize \caption{\textbf{Cross-cutting design requirements for drug discovery, therapeutic reasoning, and molecular-design agents.} The requirements distinguish workflow Function, inspectable Evidence, and their contribution to use-case-specific Validation.} \label{tab:drug_discovery_crosscutting_patterns} \setlength{\tabcolsep}{3pt} \renewcommand{\arraystretch}{1.18} \begin{tabular}{ p{0.18\linewidth} p{0.28\linewidth} p{0.28\linewidth} p{0.2\linewidth} } \hline \rowcolor{tableHeader} \textbf{Workflow requirement} & \textbf{Domain-specific principle} & \textbf{Inspectable evidence and artifacts} & \textbf{FEV interpretation} \\ \hline % ============================================================ % Requirement 1 % ============================================================ 
\rowcolor{flowAccess} Therapeutic objective and planning & Define whether the task concerns target assessment, drug repurposing, molecular design, safety analysis, treatment reasoning, trial prediction, or target-trial emulation. & Disease indication, target or drug names, molecular objectives, treatment constraints, trial protocols, cohort definitions, endpoints, analysis plans, and decision criteria. & \textbf{F1.} Planning defines the workflow but does not establish execution, therapeutic validity, or clinical utility. \\ % ============================================================ % Requirement 2 % ============================================================ 
\rowcolor{flowAccess} Therapeutic entity grounding & Resolve drugs, molecules, targets, pathways, patients, cohorts, adverse events, trial arms, and clinical endpoints using normalized and traceable representations. & SMILES strings, protein sequences, compound and target identifiers, disease ontologies, OMOP concepts, NCT identifiers, eligibility criteria, endpoints, adverse events, and cohort metadata. & \textbf{E2; E3.} Identifiable therapeutic entities and observations are necessary, but not sufficient, for replayability or scientific validity. \\ % ============================================================ % Requirement 3 % ============================================================ 
\rowcolor{flowExecution} Tool, database, and RAG execution & Query biomedical databases, knowledge graphs, molecular tools, safety resources, literature, and clinical-trial repositories using traceable inputs and explicit tool calls. & PubMed, ClinicalTrials.gov, DrugBank, ChEMBL, UniProt, Open Targets, openFDA, PubChem, PrimeKG, RTX-KG2, retrieved passages, API calls, generated SQL, tool parameters, and execution logs. & \textbf{F3; E1; E2; E4.} Execution supports V1; V2 additionally requires replayable inputs, dependencies, parameters, environments, artifacts, and traces. \\ % ============================================================ % Requirement 4 % ============================================================ 
\rowcolor{flowExecution} Prediction, screening, and molecular design & Predict, generate, prioritize, or optimize therapeutic properties, drug--target interactions, molecular structures, toxicity, treatment responses, and trial outcomes. & ADMET, HTS, DTI and drug-response datasets, generated molecules, docking poses, binding scores, toxicity predictions, synthesizability estimates, feature schemas, model outputs, SHAP values, and ranked candidates. & \textbf{E3; E4; E5.} Computational outputs support predictive and design claims, but require benchmark, robustness, statistical, or expert evaluation for V3. \\ % ============================================================ % Requirement 5 % ============================================================ 
\rowcolor{flowEvidence} Mechanistic therapeutic reasoning & Connect predictions and recommendations to biological mechanisms, drug--target relations, pathways, causal evidence, disease processes, and literature-supported rationales. & Knowledge-graph paths, mechanism-of-action reports, pathway enrichment, drug--disease relations, causal statements, Bradford--Hill-style evidence, retrieved literature, citations, and evidence-linked dossiers. & \textbf{E1; E2.} Mechanistic grounding supports interpretation and attribution but does not independently establish therapeutic efficacy or clinical benefit. \\ % ============================================================ % Requirement 6 % ============================================================ 
\rowcolor{flowEvidence} Safety and trial analysis & Evaluate adverse events, contraindications, drug interactions, cohort definitions, eligibility criteria, endpoints, causal assumptions, and statistical analysis plans. & FDA labels, openFDA records, OMOP adverse-event references, drug--drug interactions, trial protocols, generated SQL, propensity scores, IPTW outputs, clone--censor--weight analyses, Cox models, Kaplan--Meier curves, and diagnostic checks. & \textbf{E3; E4; E6.} Historical safety, pharmacological, or clinical observations contribute to Evidence but do not independently establish prospective Validation. \\ % ============================================================ % Requirement 7 % ============================================================ 
\rowcolor{flowEvidence} Critique, verification, and provenance & Detect unsupported mechanisms, invalid molecules, unsafe recommendations, weak retrieval, failed tools, code errors, and inadequate causal or trial assumptions; revise or escalate consequential outputs. & Workflow states, critic logs, repaired code, safety flags, revised protocols, retrieved citations, knowledge-graph paths, docking files, model outputs, tool traces, uncertainty statements, expert reviews, approval records, and documented limitations. & \textbf{F4; F5; F6; E4.} Critique, verification, and provenance support replay and audit, but their effectiveness must be established through task-appropriate Validation. \\ % ============================================================ % Requirement 8 % ============================================================ 
\rowcolor{flowClosure} Prospective therapeutic validation & Test an agent-generated molecule, target, mechanism, safety prediction, treatment recommendation, or trial decision using evidence aligned with the principal therapeutic or clinical claim. & Binding and functional assays, toxicity measurements, pharmacokinetic readouts, prospective preclinical studies, clinical-trial outcomes, patient follow-up, treatment-response measurements, and design-linked empirical records. & \textbf{E6; P.} V4 also requires the lower cumulative gates; \textbf{C} requires the new empirical result to change a subsequent computational, experimental, or clinical workflow action. \\ \hline \end{tabular} \vspace{0.3em} \begin{minipage}{0.98\textwidth} \footnotesize \textit{Note.} Requirements 1--6 define the core therapeutic workflow summarized in Figure~\ref{fig:drug_discovery_crosscutting_fev_blueprint}. Requirement 7 operates across that workflow, while requirement 8 is optional and claim-dependent. Archived pharmacological, preclinical, safety, or clinical observations contribute to the Evidence profile but not to prospective Validation unless an output generated by the evaluated workflow is directly tested. Independent retrospective cohorts may support qualifier \textbf{X}, but do not by themselves establish qualifier \textbf{P} or V4. \end{minipage} \end{table*}

\begin{figure*}[!t] \centering \resizebox{0.92\textwidth}{!}{% 
\begin{tikzpicture}[ x=4.45cm, y=1.0cm, core/.style={ rectangle, rounded corners, draw=blue!65!black, thick, fill=blue!7, text width=3.55cm, minimum height=1.30cm, align=center, font=\scriptsize }, evidenceband/.style={ rectangle, rounded corners, draw=green!55!black, thick, fill=green!7, text width=12.35cm, minimum height=0.92cm, align=center, font=\scriptsize }, control/.style={ rectangle, rounded corners, draw=orange!70!black, thick, fill=orange!8, text width=12.35cm, minimum height=0.88cm, align=center, font=\scriptsize }, empirical/.style={ rectangle, rounded corners, draw=red!65!black, thick, dashed, fill=red!5, text width=8.40cm, minimum height=0.96cm, align=center, font=\scriptsize }, sectionlabel/.style={ anchor=east, text width=2.20cm, align=right, font=\bfseries\scriptsize }, arrow/.style={ -{Latex[length=2mm]}, thick } ] % ============================================================ % Requirements 1--3: formulation and grounding % ============================================================ 
\node[core] (objective) at (0,0) { \textbf{1. Therapeutic objective and planning}\\[0.18em] Define the target-assessment, molecular-design, safety, treatment, or trial-analysis task }; \node[core] (entities) at (1,0) { \textbf{2. Therapeutic entity grounding}\\[0.18em] Resolve drugs, SMILES, targets, pathways, patients, cohorts, trials, endpoints, and safety events }; \node[core] (execution) at (2,0) { \textbf{3. Tool, database, and RAG execution}\\[0.18em] Query biomedical databases, knowledge graphs, molecular tools, safety resources, and trial records }; \draw[arrow] (objective) -- (entities); \draw[arrow] (entities) -- (execution); \node[ sectionlabel, text=blue!65!black ] at ([xshift=-0.35cm]objective.west) {Workflow formulation\\and grounding}; % ============================================================ % Requirements 4--6: prediction, reasoning, and safety % Snake layout: % 1 -> 2 -> 3 % | % 6 <- 5 <- 4 % ============================================================ 
\node[core] (safety) at (0,-2.20) { \textbf{6. Safety and trial analysis}\\[0.18em] Evaluate adverse events, contraindications, cohorts, endpoints, causal assumptions, and statistical plans }; \node[core] (mechanism) at (1,-2.20) { \textbf{5. Mechanistic therapeutic reasoning}\\[0.18em] Link predictions to pathways, drug--target relations, causal evidence, and literature }; \node[core] (prediction) at (2,-2.20) { \textbf{4. Prediction, screening, and molecular design}\\[0.18em] Predict or optimize efficacy, binding, ADMET, toxicity, molecules, and trial outcomes }; % Direct vertical connection from requirement 3 to requirement 4 
\draw[arrow] (execution.south) -- (prediction.north); % Snake direction: 4 -> 5 -> 6 
\draw[arrow] (prediction) -- (mechanism); \draw[arrow] (mechanism) -- (safety); \node[ sectionlabel, text=blue!65!black ] at ([xshift=-0.35cm]safety.west) {Prediction, reasoning,\\and safety}; % ============================================================ % Shared evidence and artifacts % ============================================================ 
\node[evidenceband] (artifacts) at (1,-4.00) { \textbf{Shared therapeutic evidence and artifacts:} SMILES strings, targets, molecular structures, cohort and trial metadata, retrieved passages, knowledge-graph paths, docking poses, ADMET and toxicity predictions, causal estimates, safety records, candidate rankings, and reports }; \node[ sectionlabel, text=green!45!black ] at ([xshift=-0.35cm]artifacts.west) {Shared evidence\\and artifacts}; % ============================================================ % Requirement 7: cross-cutting controls % ============================================================ 
\node[control] (control) at (1,-5.55) { \textbf{7. Critique, verification, and provenance:} preserve workflow state and traces; inspect unsupported mechanisms, invalid molecules, safety risks, failed code, causal assumptions, uncertainty, and expert-review records }; \node[ sectionlabel, text=orange!70!black ] at ([xshift=-0.35cm]control.west) {Cross-cutting\\requirements 1--6}; % ============================================================ % Requirement 8: optional prospective validation % ============================================================ 
\node[empirical] (validation) at (1,-7.15) { \textbf{8. Optional prospective therapeutic validation}\\[0.15em] Test an agent-generated molecule, target, mechanism, safety prediction, treatment recommendation, or trial decision using aligned experimental, preclinical, or clinical evidence. Closed-loop refinement requires the result to guide a subsequent action }; \node[ sectionlabel, text=red!65!black ] at ([xshift=-0.35cm]validation.west) {Optional prospective\\validation}; % ============================================================ % Background groupings % ============================================================ 
\begin{pgfonlayer}{background} \node[ rectangle, rounded corners, draw=blue!22, fill=blue!1, fit=(objective)(entities)(execution), inner sep=0.15cm ] {}; \node[ rectangle, rounded corners, draw=blue!22, fill=blue!1, fit=(safety)(mechanism)(prediction), inner sep=0.15cm ] {}; \node[ rectangle, rounded corners, draw=orange!25, fill=orange!1, fit=(control), inner sep=0.16cm ] {}; \end{pgfonlayer} \end{tikzpicture}% 
} \vspace{-0.2em} \caption{\textbf{Cross-cutting workflow blueprint for drug discovery, therapeutic reasoning, and molecular-design agents.} The core trajectory connects therapeutic-objective formulation and entity grounding with tool execution, predictive modelling, molecular design, mechanistic reasoning, and safety or trial analysis. Shared evidence includes molecular representations, target records, retrieved sources, model outputs, safety data, causal estimates, candidate rankings, and reports. Critique, verification, expert escalation, and provenance preservation operate across the workflow. Prospective therapeutic validation is optional and constitutes closed-loop refinement only when the resulting evidence guides a subsequent workflow action.} \label{fig:drug_discovery_crosscutting_fev_blueprint} \end{figure*}

\subsection{Computational Pathology, Microscopy, and Spatial Imaging Agents} 

Tables~\ref{tab:pathology_agents_infrastructure}--\ref{tab:pathology_agents_platforms} map systems spanning pathology image--text generation, bioimage infrastructure, microscopy analysis, spatial-molecular interpretation, whole-slide navigation, biomarker discovery, and cross-modal imaging automation. Representative tasks include model screening, registration, segmentation, cell quantification, region selection, multiscale diagnostic reasoning, spatial pathway analysis, prognostic modelling, and multimodal biomarker discovery. The mapped systems range from agent-readable imaging infrastructure to stateful pathology agents that execute, verify, and interpret image-analysis workflows. 

Despite this diversity, the systems share several recurring workflow requirements, summarized in Figure~\ref{fig:image_pathology_crosscutting_fev_blueprint}. Images must first be linked to their modality, tissue, magnification, assay, cohort, acquisition conditions, and biological objective. They must then be converted into inspectable regions, cells, tissue compartments, spatial neighborhoods, morphological features, or molecularly informed representations. Domain tools are subsequently executed for registration, segmentation, quantification, navigation, model adaptation, spatial analysis, and statistical modelling. Resulting claims should remain linked to identifiable image regions, molecular measurements, pathology knowledge, clinical observations, and analytical artifacts.

Workflow-state maintenance, quality control, uncertainty assessment, repair, verification, expert review, and provenance preservation operate across these activities rather than as isolated final steps. Their importance increases for diagnostic, prognostic, and biomarker-oriented outputs, where errors in registration, segmentation, region selection, magnification, cohort construction, statistical assumptions, or evidence attribution can propagate into consequential conclusions. Archived images, molecular measurements, clinical outcomes, and independent cohorts contribute to the Evidence profile or external-validation qualifier, but do not establish prospective Validation unless an output generated by the evaluated workflow is directly tested. 

Table~\ref{tab:image_pathology_crosscutting_patterns} translates these recurring patterns into domain-specific design requirements. It identifies the image inputs, tissue metadata, region and cell representations, image-analysis outputs, quality-control records, navigation traces, molecular evidence, statistical artifacts, and empirical readouts that should remain inspectable. Together, the system maps, synthesis figure, and design-requirement table separate workflow functionality, evidentiary traceability, and use-case-specific validation.

% ============================================================ % Table 21: Infrastructure and image-analysis execution % ============================================================ 
\begin{table*}[!t] \centering \footnotesize \caption{\textbf{Computational pathology, microscopy, and spatial-imaging agents: infrastructure and image-analysis execution.}} \label{tab:pathology_agents_infrastructure} \setlength{\tabcolsep}{2pt} \renewcommand{\arraystretch}{1.22} \begin{tabular}{ p{0.10\linewidth} p{0.12\linewidth} p{0.24\linewidth} p{0.24\linewidth} p{0.24\linewidth} } \hline \rowcolor{tableHeader} \textbf{System} & \textbf{Task} & \textbf{Function profile} & \textbf{Evidence profile} & \textbf{Reported V-stage and qualifiers} \\ \hline % ============================================================ % Data and model infrastructure % ============================================================ 
\flowlabel{flowAccessLabel} {Data and Model Infrastructure} \rowcolor{flowAccess} PathGen-1.6M \cite{sun2025pathgen} & Pathology image--text generation & \textit{Agent-adjacent multi-agent pipeline;} \textbf{F2, F4, F5.} Coordinates patch-selection, captioning, and revision models within a predefined data-generation workflow. & \textbf{E3, E4, E5.} WSIs, selected patches, captions, revision records, trained models, and downstream predictions. & \textbf{V3 [B,X].} The generated resource is evaluated on external pathology classification, VQA, and whole-slide benchmarks; it is not an adaptive workflow agent. \\
\rowcolor{flowAccess} BioEngine \cite{mechtel2026bioengine} & Agent-readable bioimage AI infrastructure & \textbf{F1, F3, F4, F6.} Plans service calls, screens and executes models, preserves artifacts, and rejects incompatible models. & \textbf{E2, E3, E4, E5.} BioImage.IO models, microscopy data, segmentation references, analytical outputs, execution records, and deployed applications. & \textbf{V3 [B,S,R,X].} Evaluated on HPA, PlantSeg, and Lucchi++ using model comparisons, held-out segmentation metrics, repeated fine-tuning, and external datasets. \\ \\ % ============================================================ % Microscopy and image-analysis execution % ============================================================ 
\flowlabel{flowExecutionLabel} {Microscopy and Image-Analysis Execution} \rowcolor{flowExecution} Agentic Superoptimization \cite{wangagentic} & Bioimaging workflow optimization & \textbf{F1, F3, F4, F5.} Generates preprocessing code, executes imaging workflows, evaluates downstream metrics, and iteratively revises preprocessing functions. & \textbf{E3, E4, E5.} Microscopy and medical images, generated OpenCV functions, segmentation and detection outputs, execution feedback, validation scores, and production workflow records. & \textbf{V3 [B,S,R,X].} Evaluated across spot detection, cell segmentation, and medical-image segmentation against expert and AutoML baselines, with held-out scoring, iterative optimization, and production deployment. \\ \rowcolor{flowExecution} LSM-Copilot \cite{liu2026lsm} & Fluorescence microscopy analysis & \textbf{F1, F3, F4, F5, F6.} Coordinates search, processing, and interpretation skills for microscopy loading, segmentation, quantification, evidence retrieval, repair, and reporting. & \textbf{E1, E2, E3, E4.} Microscopy files, method evidence, typed skill handoffs, segmentation and localization outputs, artifact bundles, provenance logs, and reports. & \textbf{V3 [B,S,R,X].} The same skill package is evaluated across four host settings and public 2D/3D localization benchmarks, with quantitative gains over raw-model baselines and agreement with independent Imaris measurements. \\ % ============================================================ % Spatial and molecular interpretation % ============================================================ 
\flowlabel{flowEvidenceLabel} {Spatial and Molecular Interpretation} \rowcolor{flowEvidence} QuST-LLM \cite{huang2024qust} & Spatial transcriptomics interpretation & \textbf{F1, F3, F4.} Processes selected spatial regions, extracts key genes, performs enrichment analysis, generates biological summaries, and maps text descriptions back to spatial regions. & \textbf{E1, E2, E3, E4, E5.} WSIs, Xenium data, registered regions, expression profiles, GO enrichment, selected genes, language interpretations, and region-retrieval outputs. & \textbf{V2 [B].} Executable spatial analysis is demonstrated on an identifiable Xenium dataset with reported retrieval performance. Evaluation remains limited to case-study-scale analysis. \\ \hline \end{tabular} \end{table*} % ============================================================ % Table 22: Spatial evidence and WSI navigation % ============================================================ 
\begin{table*}[!t] \centering \footnotesize \caption{\textbf{Computational pathology, microscopy, and spatial-imaging agents: spatial evidence and whole-slide reasoning.}} \label{tab:pathology_agents_reasoning} \setlength{\tabcolsep}{2pt} \renewcommand{\arraystretch}{1.22} \begin{tabular}{ p{0.10\linewidth} p{0.12\linewidth} p{0.24\linewidth} p{0.24\linewidth} p{0.24\linewidth} } \hline \rowcolor{tableHeader} \textbf{System} & \textbf{Task} & \textbf{Function profile} & \textbf{Evidence profile} & \textbf{Reported V-stage and qualifiers} \\ \hline \flowlabel{flowEvidenceLabel} {Spatial and Molecular Evidence Grounding} \rowcolor{flowEvidence} Agent SPI-WSI \cite{vashistha2025agent} & Spatial pathway inference from RNA-seq and WSI & \textbf{F1, F3, F4, F5, F6.} Generates pathway-morphology prompts, retrieves literature, incorporates pathologist critique, revises prompts, and maps approved concepts onto WSI regions. & \textbf{E1, E2, E3, E4, E5, E6.} WSIs, bulk RNA-seq and pathway scores, PubMed evidence, pathologist feedback, spatial heatmaps, manual regions, and spatial-transcriptomics observations. & \textbf{V3 [B,H,S,R,X].} Evaluated using model comparisons, pathologist scoring, manual-region agreement, hotspot ablations, and spatial-transcriptomics validation across in-house and external cohorts. The findings remain retrospective. \\ \rowcolor{flowEvidence} LAMMI-Pathology \cite{su2026lammi} & Molecularly informed pathology reasoning & \textbf{F1, F2, F3, F4, F5.} Coordinates domain-adapted tool agents, constructs grounded execution trajectories, and performs multistep image and molecular reasoning. & \textbf{E1, E2, E3, E4, E5.} Histopathology images, spatial literature, molecular APIs, tool trajectories, caption and expression-alignment outputs, and consistency and hallucination metrics. & \textbf{V3 [B,R].} Evaluated on PathSpatial-DocQA, ST-Traj, and PathMMU against agent and tool-use baselines, with trajectory, consistency, redundancy, and hallucination analyses. \\ \rowcolor{flowEvidence} CPathAgent \cite{sun2026cpathagent} & Multiscale pathology image analysis & \textbf{F1, F3, F4, F5, F6.} Screens WSIs, prioritizes regions, plans navigation, changes magnification, integrates multiscale evidence, and generates diagnostic reports. & \textbf{E2, E3, E4, E5.} WSIs, pathology reports, selected regions, navigation traces, visual representations, region descriptions, diagnostic summaries, and benchmark outputs. & \textbf{V3 [B,H,R,X].} Evaluated across patch, large-region, WSI, and out-of-distribution tasks using expert-validated questions, pathologist assessment, and component comparisons. Diagnostic trajectories remain computational. \\ \rowcolor{flowEvidence} MMNavAgent \cite{xu2026mmnavagent} & Adaptive multiscale WSI navigation & \textbf{F1, F3, F4, F5.} Selects regions and magnifications, accumulates evidence in memory, and uses iterative zoom, movement, and stopping decisions for slide diagnosis. & \textbf{E3, E4, E5, E6.} Skin WSIs, eye-tracking maps, tumor masks, selected patches, navigation histories, diagnostic predictions, and spatial-attention metrics. & \textbf{V3 [B,S,R,X].} Evaluated on 918 WSIs against fixed-magnification and navigation baselines, with classification, navigation-consistency, tumor-overlap, and cross-magnification ablation analyses. \\ \rowcolor{flowEvidence} PathAgent \cite{chen2025pathagent} & Interpretable WSI reasoning and navigation & \textbf{F1, F3, F4, F5, F6.} Selects relevant regions, extracts morphology, assesses evidence sufficiency, requests additional regions or magnification, and reports interpretable diagnostic reasoning. & \textbf{E2, E3, E4, E5.} WSIs, retrieved RoIs, multiscale patches, morphology descriptions, navigation traces, diagnostic outputs, and benchmark metrics. & \textbf{V3 [B,H,R].} Evaluated across five WSI and pathology VQA benchmarks against pathology and general vision--language models, with navigation ablations and pathologist-collaboration assessment. \\ \rowcolor{flowEvidence} WSI-Agents \cite{lyu2025wsi} & Collaborative whole-slide analysis & \textbf{F1, F2, F3, F4, F5, F6.} Routes WSI tasks to specialist agents and models, verifies outputs through logic, external knowledge, and model consensus, and produces visual reports. & \textbf{E1, E2, E3, E4, E5.} WSIs, pathology knowledge, model outputs, attention maps, verification records, consensus reports, and VQA and reporting metrics. & \textbf{V3 [B,R].} Evaluated on WSI-Bench and WSI-VQA against pathology models and agent frameworks, with ablations of allocation, verification, consensus, and summarization components. \\ \rowcolor{flowEvidence} SlideSeek + PathChat+ \cite{weishaupt2026evidencebaseddiagnosticreasoningmultiagent} & Whole-slide diagnostic reasoning & \textbf{F1, F2, F3, F4, F5, F6.} Coordinates supervisor and explorer agents to navigate WSIs, formulate diagnostic hypotheses, inspect selected regions, aggregate multiscale evidence, and draft confidence-aware reports. & \textbf{E2, E3, E4, E5.} WSIs, selected RoIs, navigation records, morphology descriptions, differential diagnoses, confidence scores, diagnostic reports, and benchmark outputs. & \textbf{V3 [B,H,R].} Evaluated on DDxBench and multiple RoI-level pathology benchmarks using diagnostic accuracy, reporting metrics, rare-disease analysis, and architecture ablations. Evaluation remains retrospective. \\ \hline \end{tabular} \end{table*} % ============================================================ % Table 23: Biomarker and spatial-biology discovery % ============================================================ 
\begin{table*}[!t] \centering \footnotesize \caption{\textbf{Computational pathology, microscopy, and spatial-imaging agents: biomarker and spatial-biology discovery.}} \label{tab:pathology_agents_discovery} \setlength{\tabcolsep}{2pt} \renewcommand{\arraystretch}{1.22} \begin{tabular}{ p{0.10\linewidth} p{0.12\linewidth} p{0.24\linewidth} p{0.24\linewidth} p{0.24\linewidth} } \hline \rowcolor{tableHeader} \textbf{System} & \textbf{Task} & \textbf{Function profile} & \textbf{Evidence profile} & \textbf{Reported V-stage and qualifiers} \\ \hline \flowlabel{flowDiscoveryLabel} {Biomarker and Spatial-Biology Discovery} \rowcolor{flowDiscovery} SPARK \cite{trost2026agentic} & Cancer-pathology biomarker discovery & \textbf{F1, F2, F3, F4, F5, F6.} Generates biological concepts, converts them into executable image-analysis parameters, verifies code and outputs, and evaluates biomarker and prognostic hypotheses. & \textbf{E2, E3, E4, E5, E6.} H\&E WSIs, spatial-proteomics data, cell and tissue masks, clinical outcomes, generated code, spatial features, survival models, SHAP values, and ranked biomarkers. & \textbf{V3 [B,S,R,X].} Evaluated retrospectively across 18 cohorts, more than 5,400 patients, five cancer types, and multiplexed spatial-imaging data, with reproducible feature extraction and prognostic modelling. \\ \rowcolor{flowDiscovery} SAGE \cite{nasser2026sage} & Knowledge-guided pathology biomarker discovery & \textbf{F1, F2, F3, F4, F5, F6.} Builds disease-specific knowledge graphs, generates and debates biomarker hypotheses, refines them with human input, discovers datasets, executes analyses, and interprets results. & \textbf{E1, E2, E3, E4, E5, E6.} Biomedical knowledge graphs, literature, multimodal patient cohorts, segmentation outputs, pathology features, survival analyses, treatment outcomes, hypotheses, debate traces, and expert scores. & \textbf{V3 [B,H,S,R].} Evaluated through hypothesis-quality assessment, debate ablations, coding-agent analysis, expert novelty and feasibility scoring, and retrospective bladder-cancer biomarker studies. Prospective clinical validation is not established. \\ \hline \end{tabular} \vspace{0.3em} \begin{minipage}{0.98\textwidth} \footnotesize \textit{Note.} Clinical outcomes and archived molecular or imaging observations contribute to the Evidence profile. Multi-cohort retrospective evaluation may support qualifiers S, R, or X, but does not establish prospective Validation of an agent-generated biomarker or prognostic claim. \end{minipage} \end{table*} % ============================================================ % Table 24: Cross-cutting pathology platforms % ============================================================ 
\begin{table*}[!t] \centering \footnotesize \caption{\textbf{Computational pathology, microscopy, and spatial-imaging agents: cross-cutting workflow platforms.}} \label{tab:pathology_agents_platforms} \setlength{\tabcolsep}{2pt} \renewcommand{\arraystretch}{1.22} \begin{tabular}{ p{0.10\linewidth} p{0.12\linewidth} p{0.24\linewidth} p{0.24\linewidth} p{0.24\linewidth} } \hline \rowcolor{tableHeader} \textbf{System} & \textbf{Task} & \textbf{Function profile} & \textbf{Evidence profile} & \textbf{Reported V-stage and qualifiers} \\ \hline \flowlabel{flowCrosscutLabel} {Cross-Cutting Pathology Platforms} \rowcolor{flowCrosscut} PathLab \cite{ma2026democratizing} & Computational pathology automation & \textbf{F1, F2, F3, F4, F5, F6.} Translates research objectives into executable pathology workflows, coordinates specialist agents, enforces methodological guardrails, and supports training, evaluation, interpretation, deployment, and reporting. & \textbf{E1, E2, E3, E4, E5, E6.} Public pathology datasets, image and clinical inputs, generated DAGs, model and segmentation outputs, survival predictions, guardrail records, execution traces, and user-study results. & \textbf{V3 [B,H,S,R,X].} Evaluated across 12 datasets and four pathology task families using prespecified non-inferiority testing, adversarial prompts, hallucination analysis, workflow timing, and studies with researchers and pathologists. \\ \rowcolor{flowCrosscut} TissueLab / TLAgent \cite{li2025co} & Cross-modal medical-imaging analysis & \textbf{F1, F2, F3, F4, F5, F6.} Plans explainable workflows across pathology, radiology, and spatial omics; executes segmentation, classification, measurement, retrieval, visualization, memory updates, and clinician-guided adaptation. & \textbf{E1, E2, E3, E4, E5, E6.} WSIs, radiology and spatial-omics data, guideline evidence, clinician annotations, segmentation and classification outputs, spatial analyses, visualizations, memory records, and execution logs. & \textbf{V3 [B,H,R,X].} Evaluated across pathology, radiology, volumetric imaging, and spatial-omics tasks with benchmark comparisons, expert feedback, visual provenance, and active-learning adaptation. Prospective deployment and outcome validation remain unestablished. \\ \hline \end{tabular} \end{table*}

\begin{table*}[!t] \centering \footnotesize \caption{\textbf{Cross-cutting design requirements for computational pathology, microscopy, and spatial-imaging agents.} The requirements distinguish workflow Function, inspectable Evidence, and their contribution to use-case-specific Validation.} \label{tab:image_pathology_crosscutting_patterns} \setlength{\tabcolsep}{3pt} \renewcommand{\arraystretch}{1.18} \begin{tabular}{ p{0.18\linewidth} p{0.28\linewidth} p{0.28\linewidth} p{0.2\linewidth} } \hline \rowcolor{tableHeader} \textbf{Workflow requirement} & \textbf{Domain-specific principle} & \textbf{Inspectable evidence and artifacts} & \textbf{FEV interpretation} \\ \hline \rowcolor{flowAccess} Image objective and context grounding & Identify the imaging modality, tissue, magnification, spatial assay, cohort, acquisition context, and biological or clinical objective. & H\&E WSIs, microscopy images, spatial-omics data, pathology reports, cohort metadata, acquisition settings, modality labels, and analysis goals. & \textbf{F1; E3.} Grounded image inputs support workflow formulation but do not independently establish replayability. \\ \rowcolor{flowAccess} Region, cell, and spatial representation & Convert images into biologically meaningful regions, cells, tissue compartments, spatial neighborhoods, and multiscale morphological features. & WSI tiles, RoIs, nuclei and cell masks, tumor/stroma regions, cell coordinates, spatial graphs, morphology captions, and marker profiles. & \textbf{E3; E5} when learned representations are used. Representation quality requires separate evaluation. \\ \rowcolor{flowExecution} Image-analysis tool execution & Execute registration, segmentation, quantification, navigation, classification, model adaptation, and spatial-analysis workflows. & QuPath, QuST, Cellpose-SAM, MCMICRO, BioImage.IO models, generated code, parameters, model checkpoints, execution logs, masks, and overlays. & \textbf{F3; E4.} Execution supports V1; V2 additionally requires replayable inputs, environments, parameters, artifacts, and traces. \\ \rowcolor{flowEvidence} Quality control and uncertainty & Assess registration, segmentation, region selection, magnification, model confidence, missing evidence, and analytical failure modes. & Registration metrics, segmentation scores, confidence estimates, QC logs, failed calls, corrected regions, uncertainty flags, and pathologist review. & \textbf{F5; F6; E4; E5.} Quality-control effectiveness must be established through benchmarks, diagnostics, robustness analysis, or expert assessment. \\ \rowcolor{flowEvidence} Biological and spatial grounding & Link image-derived observations to molecular measurements, tissue architecture, spatial organization, pathways, biomarkers, and pathology knowledge. & Spatial transcriptomics, multiplexed markers, GO terms, gene-expression outputs, biomarker labels, spatial neighborhoods, literature, and evidence-linked interpretations. & \textbf{E1; E2; E3; E6.} Molecular, pathological, or clinical observations support interpretation but do not independently establish prospective Validation. \\ \rowcolor{flowEvidence} State, navigation, and repair & Preserve image-analysis state, navigation history, region selections, tool failures, corrections, and revised analytical decisions. & Navigation traces, selected tiles, magnification histories, planner states, failed tool calls, repaired code, revised parameters, and reviewer feedback. & \textbf{F4; F5.} State and repair records support inspection and replay when the complete workflow can be reconstructed. \\ \rowcolor{flowEvidence} Provenance-preserving reporting & Report the complete image-to-evidence trajectory, including source images, regions, analytical outputs, biological interpretations, uncertainty, and limitations. & Captions, overlays, RoI coordinates, heatmaps, JSON records, code, parameters, navigation paths, model outputs, statistical results, and review records. & \textbf{F4; F6; E4.} Provenance supports replay, audit, and expert review but is not itself a scientific Validation result. \\ \rowcolor{flowClosure} Prospective biological or clinical validation & Test an agent-generated diagnosis, biomarker, spatial interpretation, prognostic claim, or imaging-derived hypothesis using evidence aligned with the principal claim. & Prospective cohorts, molecular assays, functional experiments, clinical follow-up, treatment-response evaluation, and design-linked empirical records. & \textbf{E6; P.} V4 also requires the lower cumulative gates; \textbf{C} requires the new result to change a subsequent workflow action. \\ \hline \end{tabular} \vspace{0.3em} \begin{minipage}{0.98\textwidth} \footnotesize \textit{Note.} Requirements 1--5 define the core image-to-evidence trajectory summarized in Figure~\ref{fig:image_pathology_crosscutting_fev_blueprint}. Requirements 6--7 operate across that trajectory. Requirement 8 is optional and claim-dependent. Retrospective cohorts, clinical outcomes, independent datasets, and pathologist review contribute to Evidence or Validation qualifiers but do not establish prospective Validation unless an output of the evaluated workflow is directly tested. \end{minipage} \end{table*}

\begin{figure*}[!t] \centering \resizebox{0.92\textwidth}{!}{% 
\begin{tikzpicture}[ x=4.45cm, y=1.0cm, core/.style={ rectangle, rounded corners, draw=blue!65!black, thick, fill=blue!7, text width=3.55cm, minimum height=1.30cm, align=center, font=\scriptsize }, evidenceband/.style={ rectangle, rounded corners, draw=green!55!black, thick, fill=green!7, text width=12.35cm, minimum height=0.92cm, align=center, font=\scriptsize }, control/.style={ rectangle, rounded corners, draw=orange!70!black, thick, fill=orange!8, text width=12.35cm, minimum height=0.88cm, align=center, font=\scriptsize }, empirical/.style={ rectangle, rounded corners, draw=red!65!black, thick, dashed, fill=red!5, text width=8.40cm, minimum height=0.96cm, align=center, font=\scriptsize }, sectionlabel/.style={ anchor=east, text width=2.20cm, align=right, font=\bfseries\scriptsize }, arrow/.style={ -{Latex[length=2mm]}, thick } ] % ============================================================ % Requirements 1--3 % ============================================================ 
\node[core] (context) at (0,0) { \textbf{1. Image objective and context grounding}\\[0.18em] Resolve modality, tissue, magnification, spatial assay, cohort, acquisition, and objective }; \node[core] (representation) at (1,0) { \textbf{2. Region, cell, and spatial representation}\\[0.18em] Represent regions, cells, tissue compartments, morphology, spatial neighborhoods, and scale }; \node[core] (execution) at (2,0) { \textbf{3. Image-analysis tool execution}\\[0.18em] Run registration, segmentation, quantification, navigation, classification, and spatial analysis }; \draw[arrow] (context) -- (representation); \draw[arrow] (representation) -- (execution); \node[ sectionlabel, text=blue!65!black ] at ([xshift=-0.35cm]context.west) {Image grounding\\and execution}; % ============================================================ % Requirements 4--5 % ============================================================ 
\node[core] (grounding) at (0,-2.20) { \textbf{5. Biological and spatial grounding}\\[0.18em] Link image findings to molecular measurements, tissue architecture, pathways, biomarkers, and literature }; \node[core] (quality) at (1,-2.20) { \textbf{4. Quality control and uncertainty}\\[0.18em] Check registration, segmentation, region selection, magnification, confidence, and missing evidence }; \node[ minimum width=3.55cm, minimum height=1.30cm ] (alignment) at (2,-2.20) {}; \coordinate (turn34) at (execution.south |- quality.east); \draw[arrow] (execution.south) -- (turn34) -- (quality.east); \draw[arrow] (quality) -- (grounding); \node[ sectionlabel, text=blue!65!black ] at ([xshift=-0.35cm]grounding.west) {Quality control\\and interpretation}; % ============================================================ % Shared evidence % ============================================================ 
\node[evidenceband] (artifacts) at (1,-4.00) { \textbf{Shared imaging evidence and artifacts:} WSIs, microscopy and spatial-omics data, RoIs, image tiles, cell and tissue masks, spatial coordinates, morphology features, model outputs, QC metrics, molecular measurements, biomarker records, statistical results, and reports }; \node[ sectionlabel, text=green!45!black ] at ([xshift=-0.35cm]artifacts.west) {Shared evidence\\and artifacts}; % ============================================================ % Requirements 6--7 % ============================================================ 
\node[control] (state) at (1,-5.45) { \textbf{6. State, navigation, and repair:} preserve selected regions, magnification paths, workflow state, failed calls, corrected code, revised parameters, and expert feedback }; \node[control] (reporting) at (1,-6.67) { \textbf{7. Provenance-preserving reporting:} retain source images, RoIs, overlays, navigation traces, parameters, analytical outputs, molecular evidence, uncertainty, review records, and limitations }; \node[ sectionlabel, text=orange!70!black ] at ([xshift=-0.35cm]state.west) {Cross-cutting\\controls 6--7}; % ============================================================ % Requirement 8 % ============================================================ 
\node[empirical] (validation) at (1,-8.30) { \textbf{8. Optional prospective biological or clinical validation}\\[0.15em] Test an agent-generated diagnosis, biomarker, spatial interpretation, prognostic claim, or imaging-derived hypothesis using aligned biological, experimental, or clinical evidence. Closed-loop refinement requires the result to guide a subsequent action }; \node[ sectionlabel, text=red!65!black ] at ([xshift=-0.35cm]validation.west) {Optional prospective\\validation}; % ============================================================ % Backgrounds % ============================================================ 
\begin{pgfonlayer}{background} \node[ rectangle, rounded corners, draw=blue!22, fill=blue!1, fit=(context)(representation)(execution), inner sep=0.15cm ] {}; \node[ rectangle, rounded corners, draw=blue!22, fill=blue!1, fit=(grounding)(quality), inner sep=0.15cm ] {}; \node[ rectangle, rounded corners, draw=orange!25, fill=orange!1, fit=(state)(reporting), inner sep=0.16cm ] {}; \end{pgfonlayer} \end{tikzpicture}% 
} \vspace{0.10em} \caption{\textbf{Cross-cutting workflow blueprint for computational pathology, microscopy, and spatial-imaging agents.} The core trajectory connects image and tissue-context grounding with biologically meaningful spatial representation, domain-tool execution, quality control, and evidence-linked interpretation. Shared artifacts include source images, regions, cells, spatial coordinates, analytical outputs, molecular measurements, quality metrics, and reports. State maintenance, navigation capture, repair, verification, and provenance preservation operate across the workflow. Prospective biological or clinical validation is optional and constitutes closed-loop refinement only when the resulting evidence guides a subsequent action.} \label{fig:image_pathology_crosscutting_fev_blueprint} \end{figure*}

\subsection{General Bioinformatics Workflow Agents and Automation Systems} 

Tables~\ref{tab:workflow_agents_execution}--\ref{tab:workflow_agents_discovery} map general-purpose systems spanning biomedical database access, omics analysis, biomarker discovery, executable workflow automation, biomedical machine learning, evidence verification, self-evolving tool use, and experimentally connected scientific discovery. Unlike domain-specific agents, these systems provide reusable workflow-control layers across multiple biological data types, tools, and analytical tasks. 

Despite their breadth, the systems share several recurring requirements, summarized in Figure~\ref{fig:general_workflow_crosscutting_fev_blueprint}. A biological objective must first be translated into an explicit workflow plan and routed to the appropriate data modality, tools, databases, and analytical methods. Relevant documentation, protocols, examples, and biological evidence are then retrieved to support executable code or pipeline generation. The resulting workflow should preserve its inputs, environment, parameters, intermediate artifacts, execution traces, and analytical outputs. 

Workflow-state maintenance, critique, debugging, verification, provenance capture, and escalation operate across these activities rather than as isolated final steps. Claims of generality additionally require evaluation across multiple biological domains, datasets, tools, and task formulations. Prospective testing remains uncommon; archived experimental observations contribute to the Evidence profile but do not establish prospective Validation unless an output generated by the evaluated workflow is directly tested. 

Table~\ref{tab:general_workflow_crosscutting_patterns} translates these patterns into domain-general design requirements. It identifies the workflow plans, retrieved evidence, scripts, environments, intermediate artifacts, repair traces, benchmark outputs, provenance records, and experimental readouts that should remain inspectable. Together, the system maps, synthesis figure, and design-requirement table separate workflow functionality, evidentiary traceability, and use-case-specific validation.

% ============================================================ % Table 26: Assistance and executable workflow orchestration % ============================================================ 
\begin{table*}[!t] \centering \footnotesize \caption{\textbf{General bioinformatics workflow agents: evidence access and executable workflow orchestration.}} \label{tab:workflow_agents_execution} \setlength{\tabcolsep}{2pt} \renewcommand{\arraystretch}{1.22} \begin{tabular}{ p{0.10\linewidth} p{0.12\linewidth} p{0.24\linewidth} p{0.24\linewidth} p{0.24\linewidth} } \hline \rowcolor{tableHeader} \textbf{System} & \textbf{Task} & \textbf{Function profile} & \textbf{Evidence profile} & \textbf{Reported V-stage and qualifiers} \\ \hline % ============================================================ % Assistance and evidence access % ============================================================ 
\flowlabel{flowAccessLabel} {Assistance and Evidence Access} \rowcolor{flowAccess} GFA / NagGPT \cite{cinquin2025steering} & Interactive genomics querying and analysis & \textbf{F1, F3, F5.} Rewrites invalid database requests, corrects API calls, injects warnings, and supports sequence retrieval, alignment, prediction, and exploration. & \textbf{E2, E4.} NCBI, Ensembl, UniProt and FlyBase records, transformed queries, Biopython outputs, alignments, predictions, and interaction traces. & \textbf{V1 [R].} Interactive execution and middleware-based correction are demonstrated, but silent errors remain and complete replayability is not established. \\ \rowcolor{flowAccess} BRAD \cite{pickard2025automatic} & Biomarker and enrichment workflow assistance & \textbf{F1, F3, F4, F5.} Combines document retrieval, database search, enrichment analysis, external software execution, logging, and report generation. & \textbf{E1, E2, E3, E4.} RNA-seq inputs, PubMed and arXiv passages, GO and Enrichr results, citations, JSON logs, reasoning traces, and generated reports. & \textbf{V2 [B,R].} Open workflow artifacts and action logs support replay. Evaluation includes enrichment recovery, citation accuracy, and reproducibility analyses, but the system remains primarily assistive. \\ % ============================================================ % Executable workflow orchestration % ============================================================ 
\flowlabel{flowExecutionLabel} {Executable Workflow Orchestration} \rowcolor{flowExecution} AutoBA \cite{zhou2024ai} & Autonomous omics analysis & \textbf{F1, F3, F4, F5.} Plans analyses, installs tools, writes and executes Bash workflows, records completed steps, and revises failed operations. & \textbf{E2, E3, E4.} WGS/WES, RNA-seq, scRNA-seq, ChIP-seq, ATAC-seq and spatial data; generated plans, scripts, tool outputs, logs, and reports. & \textbf{V2 [H,R].} Executable plans, code, and outputs support replay of representative workflows. Expert bioinformaticians assessed several omics use cases, but broader scientific evaluation remains limited. \\ \rowcolor{flowExecution} BioMaster \cite{su2026biomaster} & Multi-step bioinformatics automation & \textbf{F1, F2, F3, F4, F5, F6.} Coordinates planning, task execution, debugging, and checking agents; retrieves workflow knowledge, generates scripts, repairs failures, and validates intermediate outputs. & \textbf{E1, E2, E3, E4.} Multi-omics datasets, workflow and tool documentation, retrieved examples, generated scripts, execution traces, debugging logs, and checked outputs. & \textbf{V3 [B,R].} Replayable workflows are evaluated across 20 bioinformatics tasks against AutoBA and ChatGPT, with ablations of planning, tool retrieval, and checking components. \\ \rowcolor{flowExecution} Agentomics \cite{martinek2026agentomics} & Autonomous biomedical ML experimentation & \textbf{F1, F3, F4, F5, F6.} Explores datasets, selects representations and models, generates reusable code, executes iterative experiments, evaluates hidden test sets, and exports complete artifacts. & \textbf{E2, E3, E4, E5.} Twenty biomedical datasets, foundation models, generated training and inference code, containerized environments, model artifacts, deterministic metrics, and complete execution traces. & \textbf{V3 [B,S,R,X].} Evaluated through 60 runs across 20 datasets using held-out tests, triplicate execution, deterministic metrics, workflow-completion analysis, and comparisons with agentic and reported human solutions. \\ \rowcolor{flowExecution} Biomni \cite{huang2026autonomous} & General-purpose biomedical task execution & \textbf{F1, F3, F4, F5.} Composes and executes workflows over a unified biomedical action space for database querying, sequence analysis, multi-omics tasks, and tool-supported reasoning. & \textbf{E1, E2, E3, E4, E5.} Biomedical databases, sequence and omics inputs, tool calls, intermediate outputs, model predictions, workflow traces, and benchmark answers. & \textbf{V3 [B,R].} Evaluated on biomedical database, sequence, and workflow benchmarks with tool-use and task-level comparisons. Validation remains computational and depends on a largely curated action space. \\ \rowcolor{flowExecution} BioMedAgent \cite{bu2026empowering} & Self-evolving biomedical data analysis & \textbf{F1, F2, F3, F4, F5, F6.} Plans, codes, executes, repairs, and summarizes biomedical analyses while building reusable planning, coding, and tool memories. & \textbf{E1, E2, E3, E4, E5.} BioMed-AQA tasks, omics and clinical datasets, specialized tools, generated code, statistical and visualization outputs, memory records, and milestone traces. & \textbf{V3 [B,R,X].} Evaluated on 327 executable tasks and 172 knowledge questions using milestone scoring, tool and memory ablations, biomedical case studies, and external generalization to BixBench. \\ \hline \end{tabular} \end{table*} % ============================================================ % Table 27: Verification, self-evolution, and empirical discovery % ============================================================ 
\begin{table*}[!t] \centering \footnotesize \caption{\textbf{General bioinformatics workflow agents: verification, self-evolution, and experimentally grounded discovery.}} \label{tab:workflow_agents_discovery} \setlength{\tabcolsep}{2pt} \renewcommand{\arraystretch}{1.22} \begin{tabular}{ p{0.10\linewidth} p{0.12\linewidth} p{0.24\linewidth} p{0.24\linewidth} p{0.24\linewidth} } \hline \rowcolor{tableHeader} \textbf{System} & \textbf{Task} & \textbf{Function profile} & \textbf{Evidence profile} & \textbf{Reported V-stage and qualifiers} \\ \hline % ============================================================ % Verification and self-evolution % ============================================================ 
\flowlabel{flowEvidenceLabel} {Verification and Self-Evolution} \rowcolor{flowEvidence} STELLA \cite{jin2025stella} & Self-evolving biomedical research & \textbf{F1, F2, F3, F4, F5.} Coordinates manager, developer, critic, and tool-creation agents while expanding reusable reasoning templates and computational tools. & \textbf{E1, E2, E4, E5.} PubMed, ClinVar, PDB, biomedical benchmarks, model and tool outputs, reasoning templates, tool-creation records, and iterative trial traces. & \textbf{V3 [B,R].} Evaluated on biomedical knowledge, literature, and database benchmarks, with repeated computational trials showing test-time template and tool adaptation. Prospective empirical validation is not established. \\ \rowcolor{flowEvidence} Alvessa \cite{sokolova2025alvessa} & Evidence-grounded functional genomics & \textbf{F1, F2, F3, F4, F5, F6.} Recognizes entities and intent, orchestrates validated tools, generates source-grounded answers, verifies individual statements, and revises unsupported claims. & \textbf{E1, E2, E4, E5.} Functional-genomics and drug databases, retrieved records, predicted structures and pockets, citations, tool outputs, verifier feedback, and revision traces. & \textbf{V3 [B,R].} Evaluated through GenomeArena and LAB-Bench DbQA, tool-routing accuracy, statement-level provenance, adversarial verification, and drug-target assessment case studies. \\ % ============================================================ % Experimentally grounded discovery % ============================================================ 
\flowlabel{flowClosureLabel} {Experimentally Grounded Discovery} \rowcolor{flowClosure} Co-Scientist \cite{gottweis2026accelerating} & Hypothesis generation and experimental planning & \textbf{F1, F2, F4, F5, F6.} Generates, critiques, ranks, debates, and evolves scientific hypotheses through persistent memory, tournament-style comparison, and scientist oversight. & \textbf{E1, E2, E4, E5, E6.} Literature and web evidence, ranked hypotheses, debate and review traces, drug and target candidates, experimental plans, and prospective in-vitro readouts. & \textbf{V4 [B,H,R,P].} Scientist-reviewed hypotheses are connected to prospective experiments in drug repurposing, fibrosis-target discovery, and antimicrobial-resistance research. Closed-loop computational refinement from the new assay results is not consistently established. \\ \rowcolor{flowClosure} BioLab \cite{jin2025biolab} & End-to-end life-sciences research & \textbf{F1, F2, F3, F4, F5, F6.} Coordinates planning, reasoning, memory, retrieval, code execution, critique, reporting, biological models, protocol design, and experimental feedback. & \textbf{E1, E2, E3, E4, E5, E6.} Literature, xBio-Tools, biological foundation models, computational predictions, workflow traces, CRISPR measurements, antibody-assay results, and experimental reports. & \textbf{V4 [B,H,R,P].} Benchmarked against general and biomedical agents and prospectively evaluated through T-cell perturbation and PD-1 antibody assays. Physical experiments remain human-mediated, and closed-loop autonomous experimental refinement is not clearly established. \\ \hline \end{tabular} \vspace{0.3em} \begin{minipage}{0.98\textwidth} \footnotesize \textit{Note.} Prospective testing of an agent-generated hypothesis, target, perturbation, or candidate contributes qualifier P. Qualifier C should be assigned only when the resulting empirical measurement is returned to the system and changes a subsequent computational or experimental action. \end{minipage} \end{table*}

\begin{table*}[!t] \centering \footnotesize \caption{\textbf{Cross-cutting design requirements for general bioinformatics workflow agents.} The requirements distinguish workflow Function, inspectable Evidence, and their contribution to use-case-specific Validation.} \label{tab:general_workflow_crosscutting_patterns} \setlength{\tabcolsep}{3pt} \renewcommand{\arraystretch}{1.18} \begin{tabular}{ p{0.18\linewidth} p{0.28\linewidth} p{0.28\linewidth} p{0.2\linewidth} } \hline \rowcolor{tableHeader} \textbf{Workflow requirement} & \textbf{Domain-general principle} & \textbf{Inspectable evidence and artifacts} & \textbf{FEV interpretation} \\ \hline \rowcolor{flowAccess} Research objective and planning & Translate a biological question into explicit data requirements, analytical steps, dependencies, outputs, constraints, and stopping criteria. & Research goal, dataset description, task decomposition, workflow plan, expected outputs, constraints, and decision points. & \textbf{F1.} Planning defines the workflow but does not establish execution or validity. \\ \rowcolor{flowAccess} Data and task routing & Identify the biological modality and route each task to appropriate tools, databases, APIs, models, or specialist agents. & RNA-seq, ChIP-seq, WGS/WES, single-cell, spatial, protein and molecular inputs; routing decisions, tool assignments, and modality-specific metadata. & \textbf{F2; F3; E3.} Correct routing is necessary for execution but does not independently establish replayability. \\ \rowcolor{flowAccess} Evidence-grounded workflow specification & Ground analytical choices in literature, software documentation, biological databases, protocols, and validated workflow examples. & PubMed passages, database records, tool documentation, protocols, workflow examples, citations, software requirements, and retrieved evidence. & \textbf{E1; E2.} Retrieved evidence supports workflow selection and interpretation but does not itself establish Validation. \\ \rowcolor{flowExecution} Executable code and pipeline generation & Translate the grounded plan into executable scripts, notebooks, commands, or pipeline stages while managing dependencies and outputs. & Bash, Python and R code, notebooks, environments, tool calls, parameters, command histories, intermediate files, execution logs, and final artifacts. & \textbf{F3; E4.} Execution supports V1; V2 additionally requires replayable environments, inputs, parameters, artifacts, and traces. \\ \rowcolor{flowEvidence} Workflow state, critique, and repair & Maintain state, inspect failed calls and weak intermediate results, revise plans, repair code, and rerun affected workflow steps. & Shared state, critic outputs, debug logs, failed commands, corrected plans, repaired scripts, memory updates, revision histories, and tool-creation records. & \textbf{F4; F5.} Repair effectiveness must be established through benchmark, robustness, or task-appropriate scientific evaluation. \\ \rowcolor{flowEvidence} Verification and provenance preservation & Verify outputs and preserve the complete trajectory from research objective and evidence retrieval to execution, interpretation, review, and reporting. & Dataset identifiers, software versions, scripts, notebooks, logs, citations, intermediate artifacts, verification records, expert reviews, uncertainty, and limitations. & \textbf{F4; F6; E4.} Provenance supports replay and audit when the evaluated workflow can be reconstructed from reported artifacts. \\ \rowcolor{flowEvidence} Cross-domain robustness and transfer & Evaluate whether the workflow-control layer transfers across biological modalities, tools, datasets, and unseen task formulations. & Multi-domain benchmarks, unseen datasets, prompt perturbations, execution trajectories, ablations, failure analyses, external tasks, and expert comparisons. & \textbf{B; R; X} where supported. Cross-domain claims require evaluation beyond isolated demonstrations. \\ \rowcolor{flowClosure} Prospective experimental validation & Test an agent-generated hypothesis, candidate, perturbation, protocol, or intervention using evidence aligned with the principal claim. & Prioritized hypotheses, perturbation assays, CRISPR readouts, antibody assays, functional measurements, experimental reports, and feedback records. & \textbf{E6; P.} V4 also requires the lower cumulative gates; \textbf{C} requires the new empirical result to change a subsequent workflow action. \\ \hline \end{tabular} \vspace{0.3em} \begin{minipage}{0.98\textwidth} \footnotesize \textit{Note.} Requirements 1--4 define the core workflow summarized in Figure~\ref{fig:general_workflow_crosscutting_fev_blueprint}. Requirements 5--7 operate across that workflow. Requirement 8 is optional and claim-dependent. Archived experimental observations contribute to Evidence but not to prospective Validation unless an output generated by the evaluated workflow is directly tested. \end{minipage} \end{table*}

\begin{figure*}[!t] \centering \resizebox{0.92\textwidth}{!}{% 
\begin{tikzpicture}[ x=4.45cm, y=1.0cm, core/.style={ rectangle, rounded corners, draw=blue!65!black, thick, fill=blue!7, text width=3.55cm, minimum height=1.30cm, align=center, font=\scriptsize }, evidenceband/.style={ rectangle, rounded corners, draw=green!55!black, thick, fill=green!7, text width=12.35cm, minimum height=0.92cm, align=center, font=\scriptsize }, control/.style={ rectangle, rounded corners, draw=orange!70!black, thick, fill=orange!8, text width=12.35cm, minimum height=0.88cm, align=center, font=\scriptsize }, empirical/.style={ rectangle, rounded corners, draw=red!65!black, thick, dashed, fill=red!5, text width=8.40cm, minimum height=0.96cm, align=center, font=\scriptsize }, sectionlabel/.style={ anchor=east, text width=2.20cm, align=right, font=\bfseries\scriptsize }, arrow/.style={ -{Latex[length=2mm]}, thick } ] % ============================================================ % Requirements 1--3: formulation, routing, and specification % ============================================================
\node[core] (objective) at (0,0) { \textbf{1. Research objective and planning}\\[0.18em] Translate the biological goal into data requirements, analytical steps, outputs, constraints, and decisions }; \node[core] (routing) at (1,0) { \textbf{2. Data and task routing}\\[0.18em] Identify the biological modality and assign suitable tools, databases, models, APIs, or specialist agents }; \node[core] (specification) at (2,0) { \textbf{3. Evidence-grounded workflow specification}\\[0.18em] Ground analytical choices in literature, documentation, protocols, databases, and workflow examples }; \draw[arrow] (objective) -- (routing); \draw[arrow] (routing) -- (specification); \node[ sectionlabel, text=blue!65!black ] at ([xshift=-0.35cm]objective.west) {Workflow formulation\\and grounding}; % ============================================================ % Requirement 4: executable workflow generation % ============================================================ 
\node[core] (execution) at (1,-2.20) { \textbf{4. Executable code and pipeline generation}\\[0.18em] Generate and run scripts, notebooks, commands, or pipeline stages while managing dependencies and artifacts }; % Controlled elbow connection from requirement 3 to requirement 4: % downward from requirement 3, then horizontally into requirement 4 
% Requirement 3 -> requirement 4: % move downward, then point left into the right edge of requirement 4 
\coordinate (turn34) at (specification.south |- execution.east); \draw[arrow] (specification.south) -- (turn34) -- (execution.east);
\node[ sectionlabel, text=blue!65!black ] at ([xshift=-0.35cm]execution.west) {Executable workflow\\generation}; % ============================================================ % Shared evidence and artifacts % ============================================================ 
\node[evidenceband] (artifacts) at (1,-4.00) { \textbf{Shared workflow evidence and artifacts:} research goals, dataset descriptions, modality metadata, retrieved documentation, protocols, citations, workflow plans, generated scripts, software environments, intermediate files, execution logs, analytical outputs, and reports }; \node[ sectionlabel, text=green!45!black ] at ([xshift=-0.35cm]artifacts.west) {Shared evidence\\and artifacts}; % ============================================================ % Requirements 5--7: cross-cutting controls % ============================================================ 
\node[control] (repair) at (1,-5.45) { \textbf{5. Workflow state, critique, and repair:} maintain analytical state; inspect failed calls and weak intermediate results; revise plans, repair code, update memory, and rerun affected steps }; \node[control] (provenance) at (1,-6.67) { \textbf{6. Verification and provenance preservation:} retain dataset identifiers, evidence links, software versions, parameters, code, intermediate artifacts, verification outputs, uncertainty, expert-review records, and limitations }; \node[control] (transfer) at (1,-7.89) { \textbf{7. Cross-domain robustness and transfer:} evaluate workflow control across biological modalities, tools, datasets, unseen tasks, prompt variations, and external benchmarks }; \node[ sectionlabel, text=orange!70!black ] at ([xshift=-0.35cm]repair.west) {Cross-cutting\\controls 5--7}; % ============================================================ % Requirement 8: optional prospective validation % ============================================================ 
\node[empirical] (validation) at (1,-9.55) { \textbf{8. Optional prospective experimental validation}\\[0.15em] Test an agent-generated hypothesis, candidate, perturbation, protocol, or intervention using evidence aligned with the principal claim. Closed-loop refinement requires the result to guide the next action }; \node[ sectionlabel, text=red!65!black ] at ([xshift=-0.35cm]validation.west) {Optional prospective\\validation}; % ============================================================ % Background groupings % ============================================================ 
\begin{pgfonlayer}{background} \node[ rectangle, rounded corners, draw=blue!22, fill=blue!1, fit=(objective)(routing)(specification), inner sep=0.15cm ] {}; \node[ rectangle, rounded corners, draw=blue!22, fill=blue!1, fit=(execution), inner sep=0.15cm ] {}; \node[ rectangle, rounded corners, draw=orange!25, fill=orange!1, fit=(repair)(provenance)(transfer), inner sep=0.16cm ] {}; \end{pgfonlayer} \end{tikzpicture}% 
} \vspace{0.10em} \caption{\textbf{Cross-cutting workflow blueprint for general bioinformatics workflow agents.} The core trajectory connects research-objective formulation and data routing with evidence-grounded workflow specification and executable pipeline generation. Shared artifacts include retrieved evidence, scripts, software environments, intermediate files, execution logs, analytical outputs, and reports. State maintenance, repair, verification, provenance preservation, and cross-domain evaluation operate across the workflow. Prospective experimental validation is optional and becomes closed-loop refinement only when the resulting evidence guides a subsequent action.} \label{fig:general_workflow_crosscutting_fev_blueprint} \end{figure*}

\subsection{Benchmarks, Evaluation Suites, and Workflow Infrastructure} 

Tables~\ref{tab:benchmarks_evidence}--\ref{tab:benchmarks_pathology} summarize resources used to evaluate agentic bioinformatics systems. Unlike the domain-specific system tables, these resources assess whether agents can retrieve evidence, select tools, execute workflows, generate artifacts, recover from failures, preserve provenance, and produce scientifically interpretable outputs. 

The evaluation landscape spans evidence retrieval and verification, file- and code-centric workflow execution, biomedical machine learning, domain-specific analysis, tool-use trajectories, robustness testing, and long-horizon orchestration. General workflow benchmarks test whether agents can interpret task descriptions, manipulate biological files, generate and execute code, recover from errors, and reproduce graded outputs. Domain-specific benchmarks extend these criteria to genomics, gene editing, single-cell and spatial omics, protein design, drug discovery, and pathology. 

Evidence-centred resources complement executable benchmarks by testing whether biomedical claims remain linked to literature, databases, knowledge graphs, retrieved passages, entity mappings, and statement-level provenance. Process-aware resources additionally inspect tool calls, intermediate artifacts, execution traces, citation grounding, and failure recovery rather than relying only on final-answer accuracy.

Together, these resources provide the evaluation substrate for assigning use-case-specific FEV profiles and Validation stages. Demonstrated benchmark execution may support V1; replayable environments, inputs, parameters, artifacts, and traces are additionally required for V2; and V3 requires task-appropriate scientific evaluation beyond executability alone. Benchmark success does not establish V4, which requires prospective empirical testing of an output generated by the evaluated workflow.

% ============================================================ % Table 29: Evidence retrieval and general workflow evaluation % ============================================================ 
\begin{table*}[!t] \centering \footnotesize \caption{\textbf{Benchmarks and evaluation infrastructure for agentic bioinformatics: evidence retrieval and general workflow evaluation.}} \label{tab:benchmarks_evidence} \setlength{\tabcolsep}{2pt} \renewcommand{\arraystretch}{1.20} \begin{tabular}{ p{0.11\linewidth} p{0.12\linewidth} p{0.24\linewidth} p{0.27\linewidth} p{0.20\linewidth} } \hline \rowcolor{tableHeader} \textbf{Resource} & \textbf{Evaluation scope} & \textbf{What it evaluates} & \textbf{FEV contribution} & \textbf{Principal limitation} \\ \hline \flowlabel{benchEvidenceLabel} {Evidence Retrieval and Verification} \rowcolor{benchEvidence} Tool-Augmented Biomedical LLM Benchmark \cite{truong2025comprehensive} & Biomedical API and tool calling & Tests structured function calling for rsID-to-position and rsID-to-gene mapping through NCBI dbSNP and Entrez Gene across more than 100 model endpoints. & Evaluates tool selection and invocation (\textbf{F3}), integration of structured database records (\textbf{E2}), returned API outputs (\textbf{E4}), factual consistency, latency, and expert-scored correctness under multiple tool-access conditions. & Covers a small set of atomic retrieval tasks rather than complete bioinformatics workflows. \\ \rowcolor{benchEvidence} PubMed Reasoner \cite{zhang2026pubmed} & Dynamic literature retrieval and biomedical QA & Evaluates self-critical MeSH query refinement, iterative PubMed retrieval, evidence sufficiency, early stopping, and citation-grounded answer generation. & Tests retrieval planning and revision (\textbf{F1, F5}), literature grounding (\textbf{E1}), PMID-level provenance, query precision and recall, retrieval depth, answer quality, and computational cost. & Focuses on biomedical QA rather than executable molecular-data analysis or experimental workflow validation. \\ \rowcolor{benchEvidence} AMG-RAG \cite{rezaei-etal-2025-agentic} & Dynamic medical knowledge-graph retrieval & Evaluates confidence-scored entity--relation extraction, knowledge-graph construction and updating, adaptive traversal, and graph-grounded medical QA. & Supports structured evidence grounding (\textbf{E2}) through graph relations, confidence values, provenance metadata, Neo4j records, and benchmarked QA over MEDQA and MedMCQA. & Evaluation is centred on medical QA and depends on source authority, extraction quality, and expert oversight. \\ \rowcolor{benchEvidence} KGAREVION \cite{su2025kgarevion} & Biomedical knowledge-graph verification & Evaluates generation, review, and revision of biomedical triplets before answering knowledge-intensive questions from verified graph evidence. & Tests self-evaluation and repair (\textbf{F5}), structured knowledge (\textbf{E2}), inspectable triplets, UMLS mappings, graph verification, benchmark performance, generalization, and Review/Revise ablations. & Does not evaluate executable sequencing, omics, perturbation, or protein-design workflows. \\ \rowcolor{benchEvidence} DeepEvidence \cite{wang2026empowering} & Long-horizon biomedical evidence synthesis & Evaluates multi-agent exploration of literature, biomedical databases, clinical-trial resources, and APIs while constructing provenance-preserving evidence graphs. & Tests coordinated retrieval and synthesis (\textbf{F1, F2, F3, F4}), literature and structured knowledge (\textbf{E1, E2}), conflict detection, evidence-gap analysis, target prioritization, and clinical-trial reasoning. & Produces computational evidence syntheses that still require expert, experimental, or clinical evaluation. \\ \flowlabel{benchWorkflowLabel} {Process-Aware and Executable Workflow Evaluation} \rowcolor{benchWorkflow} Open-Rosalind BioBench \cite{wang2026open} & Process-aware biological-agent evaluation & Evaluates bounded tools, deterministic skills, hybrid routing, workflow-constrained execution, citation-grounded synthesis, and replayable traces across sequence and protein tasks. & Operationalizes Function through tool routing and execution (\textbf{F1, F3, F4}), Evidence through mandatory tool-derived support (\textbf{E2, E4}), and Validation support through accuracy, tool correctness, citation presence, trace completeness, and failure rate. & The benchmark is small and partly internal; external hold-out performance shows sensitivity to routing, tool coverage, and scorer normalization. \\ \rowcolor{benchWorkflow} BioML-bench \cite{miller2025bioml} & End-to-end biomedical machine learning & Tests whether agents can interpret task capsules, build data pipelines, train predictive models, and submit held-out predictions across protein, single-cell, imaging, and drug-discovery tasks. & Evaluates planning and executable model development (\textbf{F1, F3}), biological inputs and software outputs (\textbf{E3, E4, E5}), completion rates, leaderboard percentiles, AUROC, Spearman correlation, and other task-specific metrics. & Focused on supervised prediction; failures may reflect execution scaffolding rather than biological reasoning alone. \\ \hline \end{tabular} \end{table*} % ============================================================ % Table 30: General executable workflow evaluation % ============================================================ 
\begin{table*}[!t] \centering \footnotesize \caption{\textbf{Benchmarks and evaluation infrastructure for agentic bioinformatics: general executable workflow evaluation.}} \label{tab:benchmarks_general} \setlength{\tabcolsep}{2pt} \renewcommand{\arraystretch}{1.20} \begin{tabular}{ p{0.11\linewidth} p{0.12\linewidth} p{0.24\linewidth} p{0.27\linewidth} p{0.20\linewidth} } \hline \rowcolor{tableHeader} \textbf{Resource} & \textbf{Evaluation scope} & \textbf{What it evaluates} & \textbf{FEV contribution} & \textbf{Principal limitation} \\ \hline \flowlabel{benchWorkflowLabel} {General Executable Workflow Evaluation} \rowcolor{benchWorkflow} BioXArena \cite{li2026bioxarena} & Multimodal biomedical ML coding & Tests dataset inspection, representation and model selection, code generation and repair, training, and held-out prediction across 76 tasks and nine biomedical domains. & Evaluates planning, execution, and repair (\textbf{F1, F3, F5}); multimodal biological data and model outputs (\textbf{E3--E5}); hidden graders, execution traces, robustness tests, ablations, failure modes, and cost. & Performance combines biological modelling, data-interface handling, scaffold reliability, and backbone capability under a limited compute budget. \\ \rowcolor{benchWorkflow} ScienceAgent Bench \cite{chen2025scienceagentbench} & Scientific code generation & Evaluates generation of self-contained Python programs for 102 data-analysis and visualization tasks derived from 44 publications across several scientific fields. & Tests executable code production (\textbf{F3; E4}), valid execution, task success, CodeBERTScore, contamination controls, API cost, rubric-based assessment, and the effect of supplied expert knowledge. & Not specific to bioinformatics and limited to Python-centric tasks; even strong systems complete only a minority of problems. \\ \rowcolor{benchWorkflow} PromptBio-Bench \cite{guo2026promptbio} & File-centric bioinformatics workflows & Evaluates 194 expert-curated tasks spanning genomics, transcriptomics, proteomics, single-cell analysis, multi-omics, statistics, and machine learning from natural-language prompts and input files. & Tests task interpretation and execution (\textbf{F1, F3}), heterogeneous biological and computational artifacts (\textbf{E3, E4}), completion, accuracy, output-file similarity, runtime, token usage, and text or image judging. & Expert reference files may represent only one valid workflow, while LLM-based grading and single-pass evaluation can introduce bias. \\ \rowcolor{benchWorkflow} BixBench \cite{mitchener2025bixbench} & Realistic bioinformatics analysis & Evaluates 61 analysis capsules and 205 open-answer questions requiring dataset exploration, notebook execution, multistep analysis, and biological interpretation. & Tests planning, code execution, and interpretation (\textbf{F1, F3}); biological datasets and notebook artifacts (\textbf{E3, E4}); and realistic analysis trajectories rather than final-answer recall alone. & Frontier-model accuracy remains low, human baseline coverage is incomplete, and open-answer evaluation partly depends on model-based judging. \\ \rowcolor{benchWorkflow} BioAgent Bench \cite{fa2026bioagent} & Multistep bioinformatics pipelines and robustness & Evaluates ten genomics and omics workflows requiring tool use, file handling, pipeline execution, progress tracking, outcome validity, and concrete output artifacts under controlled perturbations. & Tests execution, state, and repair (\textbf{F3--F5}); biological inputs and pipeline artifacts (\textbf{E3, E4}); and robustness to prompt bloat, decoy references, corrupted inputs, model changes, and harness changes. & The relatively small task set and model-based grader limit coverage; benchmark success does not establish biological validity of downstream findings. \\ \rowcolor{benchWorkflow} BioMed-AQA \cite{bu2026empowering} & Biomedical data-analysis agents & Evaluates planning, tool selection, code execution, repair, statistics, visualization, interpretation, and reporting across 327 executable tasks and 172 knowledge questions. & Tests most Function categories (\textbf{F1--F6}) using milestone-based assessment, tool-use evaluation, repair analysis, memory ablations, and external generalization to BixBench; artifacts contribute primarily \textbf{E3--E5}. & Combines heterogeneous tasks and scoring procedures and remains limited to computational workflow competence. \\ \hline \end{tabular} \end{table*} % ============================================================ % Table 31: Genomics and single-cell evaluation % ============================================================ 
\begin{table*}[!t] \centering \footnotesize \caption{\textbf{Domain-specific agent benchmarks: genomics, gene editing, and single-cell analysis.}} \label{tab:benchmarks_omics} \setlength{\tabcolsep}{2pt} \renewcommand{\arraystretch}{1.20} \begin{tabular}{ p{0.11\linewidth} p{0.12\linewidth} p{0.24\linewidth} p{0.27\linewidth} p{0.20\linewidth} } \hline \rowcolor{tableHeader} \textbf{Resource} & \textbf{Evaluation scope} & \textbf{What it evaluates} & \textbf{FEV contribution} & \textbf{Principal limitation} \\ \hline \flowlabel{benchGenomicsLabel} {Genomics and Gene-Editing Evaluation} \rowcolor{benchGenomics} GenoTEX \cite{liu2025genotex} & Gene-expression and gene--trait analysis & Evaluates dataset selection, expression and clinical-data preprocessing, batch and confounder control, statistical workflow construction, and recovery of trait-associated genes. & Provides 1,384 problems from 911 GEO and TCGA datasets with expert workflows, intermediate artifacts, Lasso and mixed-model outputs, and reference genes. It tests planning and execution (\textbf{F1, F3}) with \textbf{E3--E5} artifacts and scientific outcome evaluation. & Restricted to transcriptomic gene--trait workflows; alternative valid preprocessing and modelling choices may differ from reference analyses. \\ \rowcolor{benchGenomics} GenomeArena \cite{sokolova2025alvessa} & Evidence-grounded functional genomics & Evaluates entity recognition, database and tool routing, evidence synthesis, statement-level provenance, verification, and revision of unsupported functional-genomics claims. & Tests planning, tools, and verification (\textbf{F1, F3, F5, F6}); literature, structured knowledge, and software outputs (\textbf{E1, E2, E4}); source-linked claims; and adversarial fabricated identifiers or numerical assertions. & Centred on database-oriented research assistance rather than raw-data bioinformatics pipelines; performance depends on database and tool coverage. \\ \rowcolor{benchGenomics} GeneEditingBench \cite{qu2026crispr} & CRISPR and gene-editing planning & Evaluates interpretation of editing objectives, CRISPR modality selection, guide and primer design, delivery reasoning, experimental constraints, specialized tool use, and downstream plans. & Tests planning, coordination, tool execution, and verification (\textbf{F1, F3, F6}) over literature, structured CRISPR knowledge, and design-tool outputs (\textbf{E1, E2, E4}). Its associated system study also reports prospectively tested editing workflows. & Cannot represent all cell-type, delivery, off-target, biosafety, and laboratory constraints; benchmark performance alone does not establish prospective validity. \\ \flowlabel{benchSpatialLabel} {Single-Cell Analysis Evaluation} \rowcolor{benchSpatial} scBench \cite{workman2026scbench} & Executable scRNA-seq analysis & Evaluates data-grounded single-cell tasks from realistic workflow snapshots, each containing a data state, natural-language instruction, and deterministic grader. & Tests planning and execution (\textbf{F1, F3}) on \textbf{E3/E4} artifacts through 394 problems, six sequencing platforms, seven task categories, deterministic grading, and task- and platform-level accuracy. & Snapshot-based tasks cover bounded analytical steps and do not establish experimental validity of newly generated findings. \\ \rowcolor{benchSpatial} Single-Cell Omics Agent Benchmark \cite{liu2026benchmarking} & Cross-framework single-cell workflows & Evaluates 50 scRNA-seq, spatial, scATAC-seq, and multi-omics tasks across multiple agent frameworks, language models, and Python or R environments. & Tests planning, tools, retrieval, execution, and repair (\textbf{F1, F3--F5}); biological and computational artifacts (\textbf{E3, E4}); 18 metrics, ground-truth scripts, robustness tests, module ablations, and failure diagnosis. & Performance depends on benchmark-specific environments, retrieval resources, reference scripts, and included analytical modules. \\ \rowcolor{benchSpatial} CellBench \cite{alber2026cellvoyager} & Published scRNA-seq workflow reproduction & Evaluates whether agents can infer, execute, and interpret analyses reported across 76 published scRNA-seq studies and extend the analyses through new hypotheses. & Tests workflow planning, execution, state, and interpretation (\textbf{F1, F3, F4}) using published dataset contexts, notebook artifacts, author-conducted analyses, and expert-reviewed trajectories. & Published analyses are neither unique nor necessarily optimal; agreement does not validate newly generated biological hypotheses. \\ \hline \end{tabular} \end{table*} % ============================================================ % Table 32: Spatial, protein, and drug-discovery evaluation % ============================================================ 
\begin{table*}[!t] \centering \footnotesize \caption{\textbf{Domain-specific agent benchmarks: spatial omics, protein design, and drug discovery.}} \label{tab:benchmarks_molecular} \setlength{\tabcolsep}{2pt} \renewcommand{\arraystretch}{1.20} \begin{tabular}{ p{0.11\linewidth} p{0.12\linewidth} p{0.24\linewidth} p{0.27\linewidth} p{0.20\linewidth} } \hline \rowcolor{tableHeader} \textbf{Resource} & \textbf{Evaluation scope} & \textbf{What it evaluates} & \textbf{FEV contribution} & \textbf{Principal limitation} \\ \hline \flowlabel{benchSpatialLabel} {Spatial and Spatial-Proteomics Evaluation} \rowcolor{benchSpatial} SpatialBench \cite{workman2025spatialbench} & Executable spatial-transcriptomics analysis & Evaluates interaction with real-world spatial data, platform-aware workflow execution, and recovery of computational and biological results using deterministic graders. & Tests planning and execution (\textbf{F1, F3}) using \textbf{E3/E4} artifacts across 146 problems, five spatial technologies, seven task categories, data snapshots, deterministic graders, models, and harnesses. & Success demonstrates bounded spatial-analysis competence rather than biological or clinical validity of new interpretations. \\ \rowcolor{benchSpatial} SP-Bench \cite{yuansp} & Spatial-proteomics workflow execution & Evaluates preprocessing, illumination correction, registration, segmentation, quantification, clustering, phenotyping, annotation, and interpretation across 102 tasks and 18 categories. & Tests domain-tool execution and workflow completion (\textbf{F3, F4}) using multiplexed tissue-imaging inputs and computational outputs (\textbf{E3, E4}), including quantification and annotation-quality metrics. & Performance depends on expert-curated skills, templates, workflow contracts, and the included spatial-proteomics tools. \\ \flowlabel{benchProteinLabel} {Protein-Design Agent Evaluation} \rowcolor{benchProtein} BioDesignBench \cite{kim2026benchmarking} & Protein-design workflow behaviour & Evaluates 76 expert-curated antibody, enzyme, binder, scaffold, and fluorescent-protein design tasks using 17 wrapped design tools and human, algorithmic, and agent baselines. & Tests planning, tool selection, design, candidate scoring, comparison, and filtering (\textbf{F1, F3, F5}) over sequences, structures, model outputs, and biophysical scores (\textbf{E3--E5}), including trace-level behaviour. & All evaluation is in silico; scoring and model-based judging do not experimentally validate generated proteins. \\ \flowlabel{benchDrugLabel} {Drug-Discovery Workflow Evaluation} \rowcolor{benchDrug} TCDD \cite{li2025drugpilot} & Drug-discovery tool calling & Evaluates tool selection, parameter extraction, structured memory, multi-function and multi-turn execution, and recovery from parameter errors using 2,800 annotated examples. & Tests routing, execution, state, and repair (\textbf{F1, F3--F5}) across eight predictive or generative drug tools, with function and parameter accuracy and controlled error scenarios. & Assesses tool-use behaviour rather than the pharmacological validity of generated molecules or predictions. \\ \rowcolor{benchDrug} PharmaBench \cite{niu2024pharmabench} & Governed therapeutic workflows & Evaluates 88 tasks covering target identification, DTI, ADMET, toxicity, drug response, preclinical reasoning, and experimental decision-making. & Tests stage-aware planning and tool use (\textbf{F1, F3}) over structured therapeutic inputs and predictions (\textbf{E3--E5}) using accuracy, F1, SMAPE, exact match, and comparisons across agents and model backbones. & Aggregate scores conflate model knowledge, tool-interface quality, and workflow orchestration; success does not establish therapeutic validity. \\ \rowcolor{benchDrug} MolBench \cite{jiang2023molbench} & Molecular screening and optimization & Evaluates molecular screening, editing, physicochemical optimization, and long-horizon structure-based discovery workflows spanning 8--50 or more steps. & Tests multistep execution, recovery, quality gates, and provenance (\textbf{F3--F5}) over molecular structures, docking outputs, property predictions, and optimized candidates (\textbf{E3--E5}), with expert rubrics and formal statistical analyses. & Evaluation remains in silico and does not establish experimental affinity, activity, toxicity, or safety. \\ \hline \end{tabular} \end{table*} % ============================================================ % Table 33: Pathology evaluation % ============================================================ 
\begin{table*}[!t] \centering \footnotesize \caption{\textbf{Domain-specific agent benchmarks: computational pathology and whole-slide reasoning.}} \label{tab:benchmarks_pathology} \setlength{\tabcolsep}{2pt} \renewcommand{\arraystretch}{1.20} \begin{tabular}{ p{0.11\linewidth} p{0.12\linewidth} p{0.24\linewidth} p{0.27\linewidth} p{0.20\linewidth} } \hline \rowcolor{tableHeader} \textbf{Resource} & \textbf{Evaluation scope} & \textbf{What it evaluates} & \textbf{FEV contribution} & \textbf{Principal limitation} \\ \hline \flowlabel{benchPathologyLabel} {Pathology Agent Evaluation} \rowcolor{benchPathology} WSI-Bench \cite{liang2025wsi} & Whole-slide morphology and reasoning & Evaluates gigapixel WSI understanding across morphology, diagnosis, treatment-oriented reasoning, reporting, and pathology VQA using 180,000 question--answer pairs from 9,850 slides and 30 cancer types. & Tests image-grounded reasoning and interpretation (\textbf{F1, F3}) using WSIs, morphology evidence, model outputs, and report artifacts (\textbf{E3--E5}), with pathology-specific precision, relevance, and VQA metrics. & It is a retrospective benchmark rather than an autonomous diagnostic workflow, and success does not establish prospective clinical validity. \\ \rowcolor{benchPathology} ST-Traj \cite{su2026lammi} & Pathology tool-execution trajectories & Evaluates tool selection and ordering, intermediate-observation interpretation, trajectory consistency, redundant calls, hallucination, and answer agreement over 6,818 multistep trajectories. & Tests execution, state maintenance, and verification (\textbf{F3, F4, F6}) using grounded tool interactions and computational traces (\textbf{E4}), including Tool Consistency F1, Trajectory Success, Answer Consistency, redundancy, and hallucination metrics. & Higher-level trajectories are partly model-assembled and bounded by the included pathology and molecular tools. \\ \rowcolor{benchPathology} DDxBench \cite{weishaupt2026evidencebaseddiagnosticreasoningmultiagent} & Whole-slide differential diagnosis & Evaluates WSI navigation, region and magnification selection, iterative diagnostic refinement, multiregion evidence integration, and visually grounded reports across 150 slides and 55 neoplastic diseases. & Tests planning, navigation, state, and verification (\textbf{F1, F3, F4, F6}) using WSI regions, morphology evidence, confidence values, diagnostic outputs, pathologist review, architecture ablations, and failure analysis. & The benchmark is small, single-institution, non-public, and limited to neoplastic diagnoses; retrospective accuracy does not establish clinical deployment validity. \\ \hline \end{tabular} \vspace{0.3em} \begin{minipage}{0.98\textwidth} \footnotesize \textit{Note.} Benchmark and evaluation resources are not assigned independent V-stages in these tables. Instead, they provide evidence for classifying evaluated system use cases. Demonstrated benchmark execution may support V1; V2 additionally requires sufficient environments, inputs, parameters, artifacts, and traces for replay; and V3 requires task-appropriate scientific evaluation. Benchmark comparisons, expert assessment, statistical analysis, robustness testing, and external evaluation may be recorded through qualifiers \textbf{B}, \textbf{H}, \textbf{S}, \textbf{R}, and \textbf{X}, respectively. Benchmark performance alone does not establish prospective empirical Validation, qualifier \textbf{P}, or V4. \end{minipage} \end{table*}

\newpage
\clearpage
% \end{document}
